# Supplementary material for: Learning Temporal Point Processes for Efficient Retrieval of Continuous Time Event Sequences
Source: arXiv:2202.11485 source file (2022-02-17)
Supplement: Supplementary file 1 [file 080appendix.tex]

\begin{center}
 \Large{\bf Appendix\\
(Learning Temporal Point Processes for Efficient Retrieval\\ of Continuous Time Event Sequences)}
\end{center}

\section{Background: Marked Temporal Point Processes} \label{app:back}
Marked Temporal point processes (MTPP) are probabilistic generative models for continuous-time event sequences. MTPP can be represented as a probability distribution over sequences of variable lengths belonging to a time interval $[0, T]$. Therefore, they can be realized as an event sequence $\mathcal{S}_k = \{(t_1, m_1 ), \cdots (t_N , m_N)\}$, where $N$ is the number of events. Here, the times are ever-increasing \ie\ $0 < t_1 < \cdots < t_N \le T$ and $m_i \in \mathcal{C}$ is the corresponding mark with $\mathcal{C}$ as the set of all categorical marks. A MTPP can be characterized by its conditional intensity function, $\lambda^*(t)$. The $*$ denotes a dependence on the history. Given the conditional intensity function, we can obtain the conditional probability density function (PDF) as:
\begin{equation}
p^*(\Delta_{t, i}) = \lambda^*(t_{i-1} + \Delta_{t, i}) \exp \big(-\int_{0}^{\Delta_{t, i}} \lambda^*(t_{i-1} + r) dr\big)
\end{equation}
where $\Delta_{t, i}$ denotes the inter-event time interval \ie, $t_i - t_{i-1}$.

\noindent In recent years, neural enhancements to MTPP models have significantly enhanced the predictive power of these models. Specifically, they combine the continuous-time approach from the point process with deep learning approaches and thus can better capture complex relationships between events. The most popular approaches~\cite{du2016recurrent, MeiE16, shchur2019intensity, zhang2019self, zuo2020transformer} use different methods to model the time- and mark-distribution via neural networks. Specifically,~\cite{du2016recurrent} embeds the event history to a vector representation via a recurrent encoder that updates its state after parsing each event in a sequence; ~\cite{MeiE16} modified the LSTM architecture to employ a continuous-time state evolution; ~\cite{shchur2019intensity} replaced the intensity function with a mixture of \textit{Log-Normal} flows for closed-form sampling;~\cite{zhang2019self} utilized the transformer architecture\cite{vaswani2017} to capture the long-term dependencies between events in the history embedding and \cite{zuo2020transformer} used the transformer architecture for sequence embedding but extended it to graph settings as well. However, these models were designed to capture the generative distribution of future events in sequences, rather than the relevance between sequences. Thus, these models cannot be extended to the problem of sequence retrieval.

\section{Hashing}\label{app:hashing}

\subsection{Random hyperplane based hashing method}
% \label{sec:rh}
Since the relevance between the query and corpus sequence pairs $(\Hcal_q,\Hcal_c)$ is measured using the cosine similarity between the gradient vectors, \ie, $\kernel_{p_{\theta}}(\Hcal_q,\Hcal_c)$\eat{$\textsc{CosSim}(\vb_{p_{\theta}} (U(\Hcal_q)), \vb_{p_{\theta}} (\Hcal_c))$}, one can use random hyperplane based locality sensitive hashing method for hashing the underlying gradient vectors $\vb_{p_{\theta}} (\Hcal_c)$~\cite{charikar2002similarity}.
Towards this goal, after training \ourf\, %once we train a \ourf\ model $p_{\theta}$, we build the binary hash codes from the trained vectors $ \vb_{p_{\theta}}(\Hcal_c)$ of the corpus sequences.
%More in details, 
we generate $R$ unit random vectors $\ub_r\in \RR^D$ from i.i.d. Normal distributions and then compute a binary hash code
$\hash^c = [\sgn (\ub_1 ^\top \vb_{p_{\theta}}(\Hcal_c)),\dots, \sgn (\ub_R ^\top \vb_{p_{\theta}}(\Hcal_c))] $ for each $c\in \Ccal$. This leads to $2^R$ possible hash buckets $\set{\Bcal}$, where
each corpus sequence is assigned to one hash bucket using the algorithm proposed by~\citet{GionisIM1999hash}. %It should be noted that since the hash codes are computed prior to observing the query sequence, we cannot use \ours\ to compute $\vb^c$ as it requires the presence of the corresponding query sequence $\Hcal_q$.

When we encounter an unseen test query $\Hcal_q$,  we compute the corresponding hash code $\hash^q$, assign it to a bucket $\Bcal$ and finally return \emph{only those sequences} $\Hcal_c$ which were assigned to this bucket $\Bcal$. Thus, for each query, the number of comparisons is reduced from $|\Ccal|$ to $|\Bcal|$, \ie, the number of corpus sequences in the bucket $\Bcal$.
Thus, if the corpus sequences are assigned uniformly across the different buckets, then the expected number of comparisons becomes $|\Ccal|/2^R$, which provides a significant improvement for  $R>2$. 

\xhdr{Limitations} In practice, binary hash codes are not trained from data and consequently, they are not optimized
to be uniformly distributed across different hash buckets. Consequently, the assignment of corpus sequences across different buckets may be
quite skewed, leading to inefficient sequence retrieval.

\subsection{Details about our proposed hashing method}
As suggested in~\cite{GionisIM1999hash}, we design multiple hash tables and assign a bucket to the hashcode of a sequence using only a set of bits selected randomly. More specifically, let the number of hash-tables be $M$. Given a query sequence, we calculate its hashcode using the procedure described in Algorithm~\ref{alg:key}, $\hash^{\newq} = \sgn\left(\Lambda_{\psi}(\vb^{\newq})\right)$. The hash code is a $R$ dimension vector with $\hash^{\newq} \in \{-1, 1\}^{R}$ and from this vector, we consider $L$ bits at random positions to determine the bucket to be assigned to the sequence. Here, $\hash^{\newq} $ represent the numbers between $\{0, 2^{L}-1\}$, \ie,  one of the $2^{L}$ different buckets in a hash table. Correspondingly, we assign $\hash^{\newq}$ into a bucket. However, such a procedure is dependent on the specific set of bits --that were selected randomly-- used for deciding the bucket-ID. Therefore, we use $M$ hash-tables and repeat the procedure of sampling $L$ bits and bucket assignment for each table. We follow a similar bucket assignment procedure for corpus sequences. As described in Algorithm~\ref{alg:key}, for an incoming query sequence in the test set, we use the above bucket assignment procedure and compute the relevance score for only the corpus sequences within the same buckets. For all our experiments we set $H$ same as the hidden dimension $D$, $M = 10$, and $L=12$.

\section{Additional details about the experimental setup}\label{app:imp_details}
In this appendix, we elaborate on the details of dataset characteristics, evaluation metrics, and hardware configuration.

\begin{table}[t]
\small
	\centering
	\begin{tabular}{l|ccccc}
	\toprule
	\textbf{Dataset} & \textbf{Audio} & \textbf{Celebrity} & \textbf{Electricity} & \textbf{Health} & \textbf{Sports}\\ \hline
	$  {|\Cr_{q\rel}|}/{|\Cr|} $ & 0.25 & 0.23 & 0.20 & 0.28 & 0.30\\
	Total Events & 1M & 50M & 60M & 60M & 430k \\
	\# Marks & 5 & 16 & 5 & 5 & 21 \\
	\bottomrule
	\end{tabular}
 	\caption{Statistics of the search corpus for all datasets. ${|\Cr_{q\rel}|}/{|\Cr|}$ denotes the ratio of positive corpus sequences to the total sequences sampled for training. The ratio is kept same for all queries.}\vspace{1mm}
	\label{tab:dset_details}
\end{table}

\subsection{Dataset Statistics}
We evaluate the retrieval performance of \our and other methods across large-scale real-world datasets with up to 60 million events. The statistics of all datasets are given in Table~\ref{tab:dset_details}. Across all datasets, $|\Hcal_q| = 5K$ and $|\Hcal_c| = 200K$. We partition the set of queries into 50\% training, 10\% validation, and the rest as test sets. During training, we negatively sample 100 corpus sequences for each query.

\begin{asparaenum}[(1)]
\item \textbf{Audio:} The dataset contains audio files for spoken commands to a smart-light system and the demographics(age, nationality) of the speaker.  Here, a query corpus sequence pair is relevant if they are from an audio file with a common speaker.

\item \textbf{Sports:} The dataset contains actions (\eg run, pass, shoot) taken while playing different sports. We consider the time of action and action class as time and mark of sequence respectively. Here, a query corpus sequence pair is relevant if they are from a common sport.

\item \textbf{Celebrity:} In this dataset, we consider the series of frames extracted from youtube videos of multiple celebrities as event sequences where event-time denotes the video-time and the mark is decided upon the coordinates of the frame where the celebrity is located.
Here, a query corpus sequence pair is relevant if they are from a video file having a common celebrity.
% We consider the video sequences with a common celebrity as relevant. 

\item \textbf{Electricity:}  This dataset contains the power-consumption records of different devices across smart-homes in the UK. We consider the records for each device as a sequence with event mark as the \textit{normalized} change in the power consumed by the device and the time of recording as event time. 
Here, a query corpus sequence pair is relevant if they are from a  similar appliance.
% The sequences from a similar appliance are considered relevant.

\item \textbf{Health:} The dataset contains ECG records for patients suffering from heart-related problems. Since the length of the ECG record for a single patient can be up to 10 million, we generate smaller individual sequences of length 10,000 and consider each such sequence as an independent sequence. The marks and times of events in a sequence are determined using a similar procedure as in Electricity. 
Here, a query corpus sequence pair is relevant if they are from a common patient.
\end{asparaenum}

For Health, Celebrity and Electricity, we lack the true ground-truth labeling of relevance between sequences. Therefore, we adopt a heuristic in which, given a dataset $\Dcal$, from each sequence $\seq_q\in\Dcal$ with $q\in[|\Dcal|]$, we first sample a set of sub-sequences $\mathcal{U}_q=\set{\Hcal\subset \texttt{seq}_q}$ with $|\Ucal_q|\sim \text{Unif}\,[200,300]$. For each such collection $\Ucal_q$, we draw exactly one query $\Hcal_q$ uniformly at random from $\Ucal_q$, \ie, $\Hcal_q\sim\Ucal_q$. Then, we define $\Cr=\cup_{q\in[|\Dcal|]}\Ucal_q\cp \Hcal_q$, $\Cr_{q\rel}=\Ucal_q\cp \Hcal_q$ and $\Cr_{q\nrel}=\cup_{c\neq q}\big(\Ucal_c\cp \Hcal_c\big)$.

\subsection{System Configuration}
All our models were implemented using Pytorch v1.6.0~\footnote{https://pytorch.org/}. We conducted all our experiments on a server running Ubuntu 16.04, CPU: Intel(R) Xeon(R) Gold 6248 2.50GHz, RAM: 377GB, and GPU: NVIDIA Tesla V100. 

\subsection{Hyperparameters setup}
We set the hyper-parameters values of \our\ as follows: \begin{inparaenum}[(i)] \item contribution of model-independent similarity score in Eq.~\eqref{eq:relevance-score-function}, $\gamma = 0.1$; \item margin parameters for parameter estimation, $\delta \in \{0.1, 0.5, 1\}$ and weight for constraint violations, $\lambda \in \{0.1, 0.5, 1\}$; \item weight parameters for hashing objective~\eqref{eq:hash} $\eta_1, \eta_2, \eta_3 \in \{0.1, 0.2, 0.25\}$ and correspondingly $\eta_4 \in \{0.25, 0.4, 0.7\}$. 
\end{inparaenum}
\begin{table}[tbh]
\small
\centering
	\begin{tabular}{lccccc}
	\toprule
	\multirow{2}{*}{\textbf{Parameters}} & \multicolumn{5}{c}{\textbf{Datasets}} \\
	\cmidrule(lr){2-6}
	& \textbf{Audio} & \textbf{Celebrity} & \textbf{Electricity} & \textbf{Health} & \textbf{Sports}\\ \midrule
	$\gamma$ & 0.1 & 0.1 & 0.5 & 0.1 & 0.1\\
	$\delta$ & 0.5 & 0.5 & 0.1 & 0.1 & 0.5\\
	$\{\eta_1, \eta_2, \eta_3\}$ & \{0.4, 0.3, 0.3\} & \{0.4, 0.3, 0.3\} & \{0.4, 0.3, 0.3\} & \{0.5, 0.25, 0.25\} & \{0.5, 0.25, 0.25\} \\
	Batch-size $\mathcal{B}$ & 32 & 32 & 32 & 16 & 16\\
	$D$ & 64 & 64 & 48 & 32 & 32\\
	\bottomrule
	\end{tabular}
\caption{Hyper-parameter values used for different datasets. The values are determined by fine-tuning the performance on the validation set.}
\label{tab:hyperparameters}	
\end{table}

Moreover, the values of training specific parameter values are: \begin{inparaenum}[(i)] \item batch-size, $\mathcal{B}$ is selected from $\{16, 32\}$, \ie for each batch we select $\mathcal{B}$ query sequences and all corresponding corpus sequences; \item hidden-layer dimension for cross-attention model, $D \in \{32, 48, 64\}$; \item number of attention blocks $N_b = 2$; \item number of attention heads $N_h = 1$ and \item UMNN network as a 2 layer feed-forward network with dimension $\{128, 128\}$. \end{inparaenum} We also add a dropout after each attention layer with probability $p = 0.2$ and an $l_2$ regularizer with over the trainable parameters with the coefficient set to $0.001$. All our parameters are learned using the Adam optimizer. We summarize the details of hyperparameters across different datasets in Table~\ref{tab:hyperparameters}.

\subsection{Evaluation metrics}
We evaluate \our and the baselines using mean average precision (MAP), NDCG@k, and mean reciprocal rank (MRR). We calculate these metrics as follows:
\begin{equation}
\text{MAP} = \frac{1}{|\Hcal_{q'}|}\sum_{q' \in \Hcal_{q'}} \text{AP}_{q'}, \quad \text{NDCG@k} = \frac{\text{DCG}_k}{\text{IDCG}_k}, \quad \text{MRR} = \frac{1}{|\Hcal_{q'}|} \sum_{q' \in \Hcal_{q'}}\frac{1}{r_{q'}},
\end{equation}
where $\text{AP}_{q'}, \text{DCG}_k, \text{IDCG}_k$, and $r_{q'}$ denote the average precision, discounted cumulative gain at top-$k$ position, ideal discounted cumulative gain (at top-$k$), and the topmost rank of a related corpus sequence respectively. For all our evaluations, we follow a standard evaluation protocol~\cite{sasrec, tisasrec} for our model and all baselines wherein for each query sequence in the test set, we rank all relevant corpus sequence and 1000 randomly sampled non-relevant sequences. All confidence intervals and standard deviations are calculated after 5 independent runs. For all metrics -- MAP, NDCG, and MRR, we report results in terms of percentages with respect to maximum possible value \ie 1.

\subsection{Baseline Implementations}
For all the baselines, we use the official python implementations released by the authors of MASS~\footnote{https://www.cs.unm.edu/$\sim$mueen/MASS.py}, UDTW~\footnote{https://github.com/klon/ucrdtw}, Sharp~\footnote{https://github.com/google-research/soft-dtw-divergences}, RMTPP~\footnote{https://github.com/Networks-Learning/tf\_rmtpp}, SAHP~\footnote{https://github.com/QiangAIResearcher/sahp\_repo}, and THP~\footnote{https://github.com/SimiaoZuo/Transformer-Hawkes-Process} and we thank them for making their codes public. For MASS and UDTW, we report the results using the default parameter values. For Sharp, we tune the hyper-parameter `\textit{gamma}' (for more details see~\cite{blondel2021differentiable}) based on the validation set. In RMTPP, we set the BPTT length to 50, the RNN hidden layer size to 64, and the event embedding size 16. These are the parameter values recommended by the authors. For SAHP and THP, we set the dimension to 128 and the number of heads to 2. The values for all other transformer parameters are similar to the one we used for the attention-part in \our.

\begin{table*}[t!]
\footnotesize
\centering
\begin{tabular}{l|ccccc}
\toprule
\textbf{Dataset} & \multicolumn{5}{c}{\textbf{Mean Reciprocal Rank (MRR)}} \\ \hline 
 & Audio & Celebrity & Electricity & Health & Sports\\ \hline \hline
MASS~\cite{mass} & 57.3$\pm$0.0 & 63.7$\pm$0.0 & 17.6$\pm$0.0 & 27.2$\pm$0.0 & 61.6$\pm$0.0\\
UDTW~\cite{ucrdtw} & 58.5$\pm$0.0 & 64.8$\pm$0.0 & 18.7$\pm$0.0 & 29.2$\pm$0.0 & 61.2$\pm$0.0\\
Sharp~\cite{blondel2021differentiable} & 58.7$\pm$1.7 & 65.4$\pm$2.6 & 19.8$\pm$0.6 & 30.4$\pm$0.7 & 61.1$\pm$2.3\\
RMTPP~\cite{du2016recurrent} & 54.2$\pm$3.9 & 64.5$\pm$4.6 & 15.8$\pm$1.2 & 25.2$\pm$1.8 & 56.2$\pm$4.8\\
\texttt{Rank}-RMTPP & 60.8$\pm$3.7 & 65.6$\pm$4.0 & 23.3$\pm$1.5 & 30.7$\pm$1.7 & 62.7$\pm$3.9\\
SAHP~\cite{zhang2019self} & 56.9$\pm$4.3 & 64.2$\pm$4.8 & 17.2$\pm$1.3 & 26.7$\pm$2.1 & 59.4$\pm$4.9\\
\texttt{Rank}-SAHP & 60.3$\pm$2.5 & 66.1$\pm$2.9 & 25.9$\pm$1.2 & 32.6$\pm$1.4 & 62.1$\pm$2.9\\
THP~\cite{zuo2020transformer} & 58.6$\pm$2.6 & 65.0$\pm$2.9 & 20.1$\pm$1.1 & 28.2$\pm$1.3 & 60.9$\pm$3.3\\
\texttt{Rank}-THP & 62.2$\pm$2.8 & 68.9$\pm$3.0 & 31.4$\pm$1.4 & 36.2$\pm$1.7 & 63.4$\pm$2.9\\
\ourf & 63.6$\pm$2.7 & 69.3$\pm$3.1 & 33.4$\pm$1.6 & 37.9$\pm$1.7 & 64.3$\pm$3.1\\
\ours & \textbf{64.5$\pm$2.9} & \textbf{70.1$\pm$3.3} & \textbf{35.2$\pm$1.7} & \textbf{40.3$\pm$1.9} & \textbf{66.7$\pm$3.1}\\
\bottomrule
\end{tabular}
\caption{Retrieval quality in terms of mean reciprocal rank(MRR in \%) of  all the methods across five datasets on the test set. Numbers with bold font (underline) indicate best (second best) performer. Boxed numbers indicate best performing state-of-the-art baseline.}
\label{tab:exp_mrr}
\centering
\begin{tabular}{l|ccccc}
\toprule
\textbf{Dataset} & \multicolumn{5}{c}{\textbf{NDCG@20}} \\ \hline 
 & Audio & Celebrity & Electricity & Health & Sports\\ \hline \hline
MASS~\cite{mass} & 17.5$\pm$0.0 & 31.4$\pm$0.0 & 8.1$\pm$0.0 & 13.5$\pm$0.0 & 16.3$\pm$0.0\\
UDTW~\cite{ucrdtw} & 17.9$\pm$0.0 & 32.5$\pm$0.0 & 8.8$\pm$0.0 & 14.4$\pm$0.0 & 16.0$\pm$0.0\\
Sharp~\cite{blondel2021differentiable} & 18.2$\pm$0.5 & 33.6$\pm$0.7 & 11.9$\pm$0.3 & 15.9$\pm$0.4 & 17.2$\pm$0.7\\
RMTPP~\cite{du2016recurrent} & 16.0$\pm$1.1 & 32.2$\pm$1.6 & 7.1$\pm$0.5 & 12.1$\pm$0.7 & 17.1$\pm$1.1\\
\texttt{Rank}-RMTPP & 20.2$\pm$1.0 & 33.4$\pm$1.4 & 10.5$\pm$0.5 & 15.4$\pm$0.6 & 21.8$\pm$1.2\\
SAHP~\cite{zhang2019self} & 19.8$\pm$1.4 & 31.7$\pm$2.1 & 7.8$\pm$0.5 & 13.1$\pm$0.9 & 19.2$\pm$1.5\\
\texttt{Rank}-SAHP & 21.5$\pm$0.9 & 34.1$\pm$1.0 & 12.3$\pm$0.4 & 17.4$\pm$0.6 & 22.9$\pm$1.0\\
THP~\cite{zuo2020transformer} & 19.7$\pm$0.8 & 32.9$\pm$1.0 & 9.5$\pm$0.4 & 14.4$\pm$0.5 & 20.8$\pm$0.9\\
\texttt{Rank}-THP & 21.8$\pm$0.9 & 37.7$\pm$1.2 & 14.4$\pm$0.6 & 19.3$\pm$0.6 & 23.3$\pm$1.1\\
\ourf & 22.9$\pm$1.3 & 40.3$\pm$1.5 & 16.3$\pm$0.7 & 20.9$\pm$1.0 & 23.8$\pm$1.6\\
\ours & \textbf{24.2$\pm$1.5} & \textbf{42.0$\pm$1.8} & \textbf{17.6$\pm$0.8} & \textbf{22.3$\pm$1.0} & \textbf{25.7$\pm$1.7}\\
\bottomrule
\end{tabular}
\caption{Retrieval quality in terms of NDCG@20 (in \%) of  all the methods across five datasets on the test set. Numbers with bold font (underline) indicate best (second best) performer. Boxed numbers indicate best performing state-of-the-art baseline.}
\label{tab:exp_n20}
\end{table*}

% \newpage
\section{Additional experiments with real data}\label{app:expts}
\subsection{Analysis of Retrieval Accuracy}
In addition to results in Table~\ref{tab:main}, we evaluate the performance of \our and all baselines through mean reciprocal rank (MRR) and NDCG@20, given in Table~\ref{tab:exp_mrr} and Table~\ref{tab:exp_n20} respectively. These results show that \our outperforms all other baseline models across different evaluation metrics. Moreover, in contrast to Table~\ref{tab:main}, we note that \our outperforms \tpprank-THP in both MRR and NDCG@20 metrics.

\subsection{Analysis at a query level} 
Next, we compare the performance between \our and other state-of-the-art methods, at a query level.  Specifically, for each query $\Hcal_q$ we compute the advantage of using \our in terms of gain in average precision, i.e., AP(\our) $-$ AP(baseline) for two most competitive baselines -- \tpprank-SAHP and \tpprank-THP.  We summarize the results in Figure~\ref{fig:app_drill}, which show that for at least 70\% of the queries, \our outperforms or fares competitively with these baselines, across all datasets.
\begin{figure}[t]
\centering
{\includegraphics[height=2.2cm]{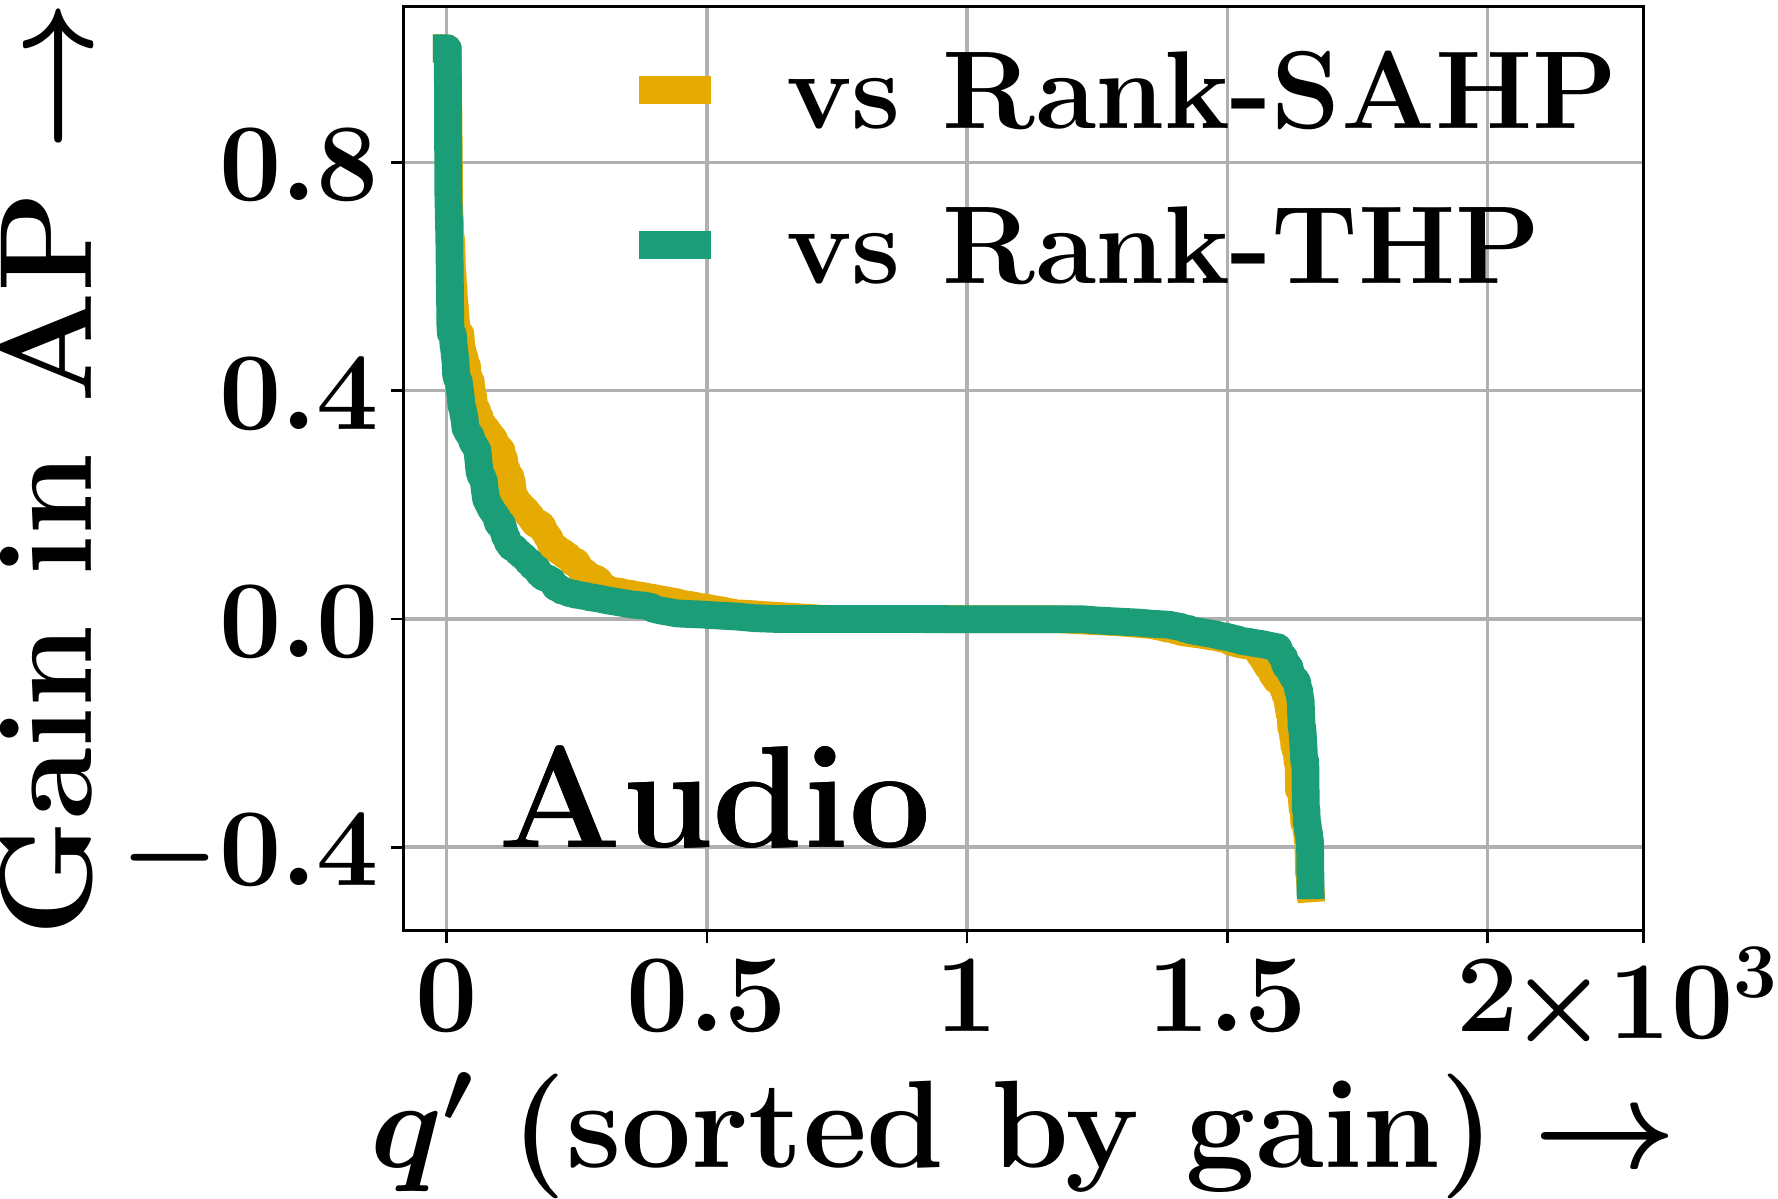}}
{\includegraphics[height=2.2cm]{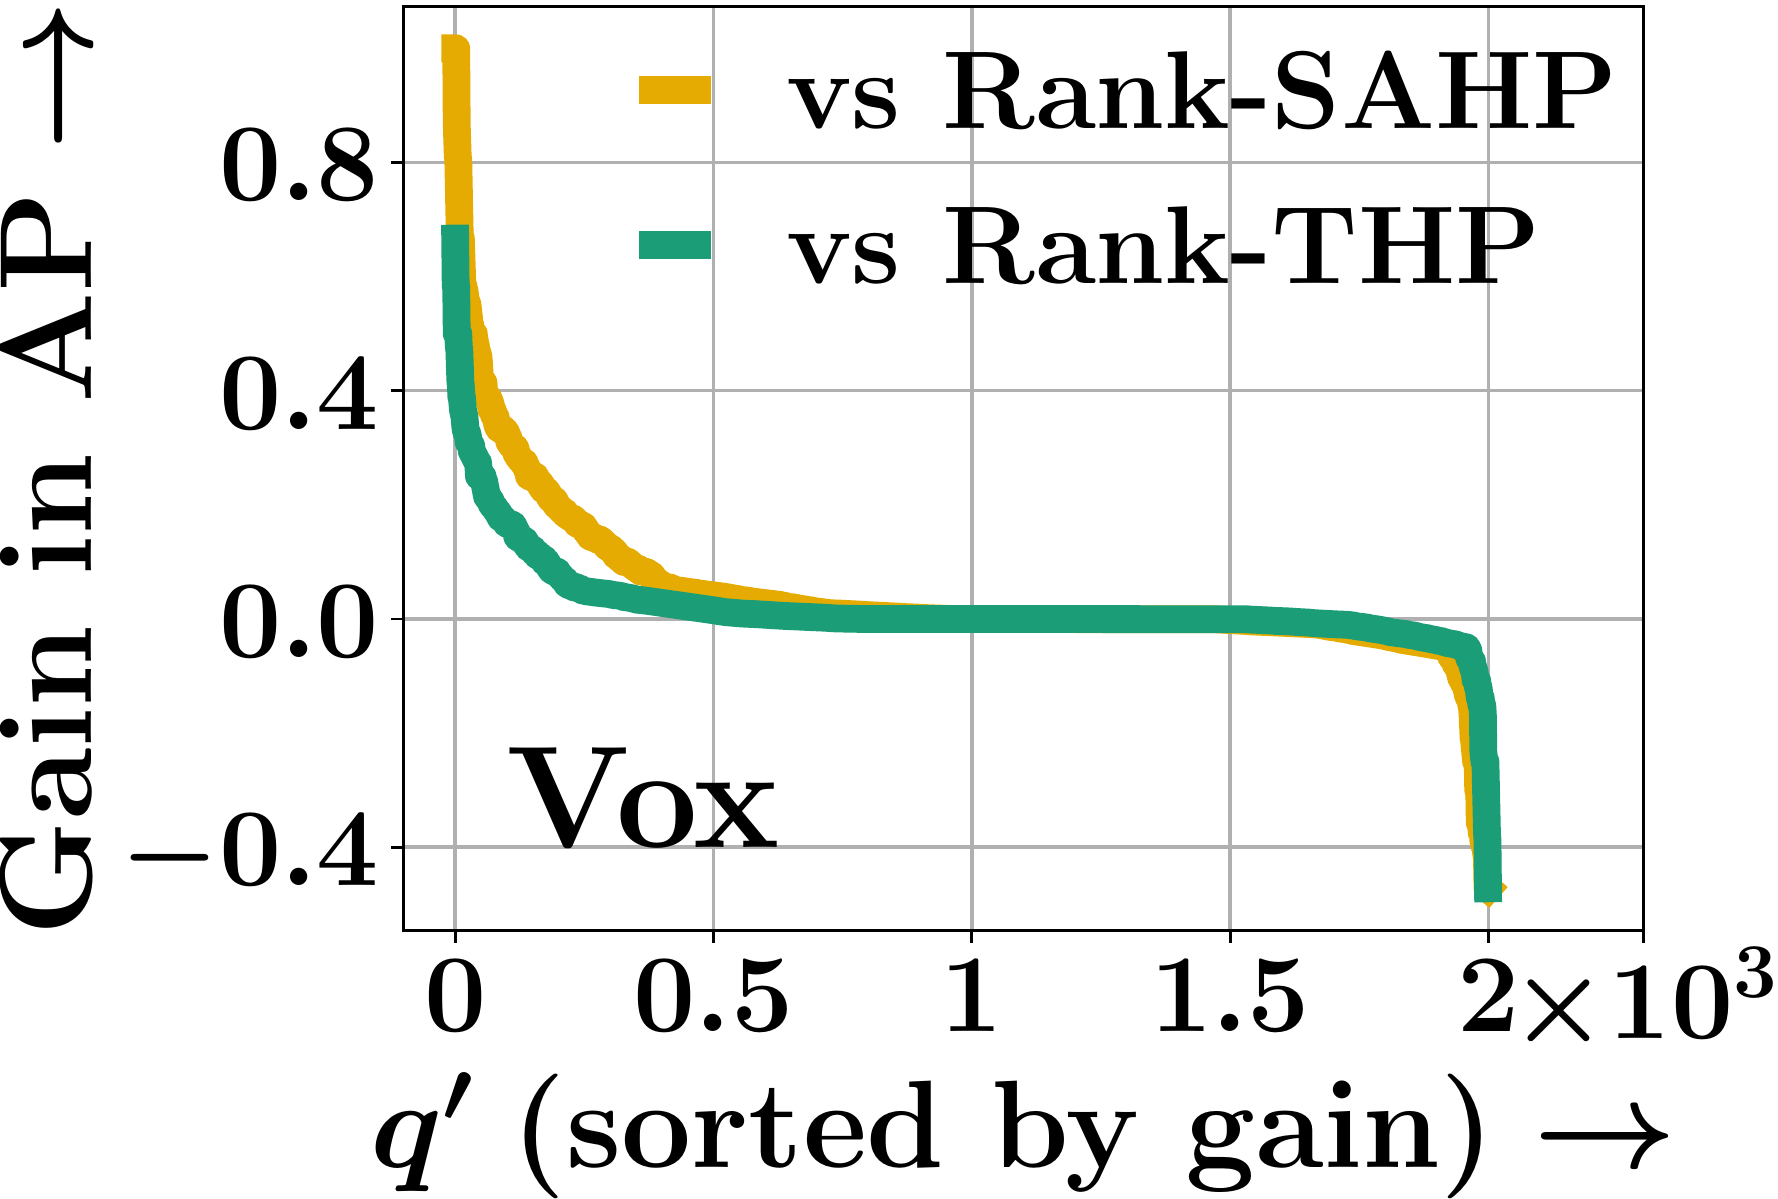}}
{\includegraphics[height=2.2cm]{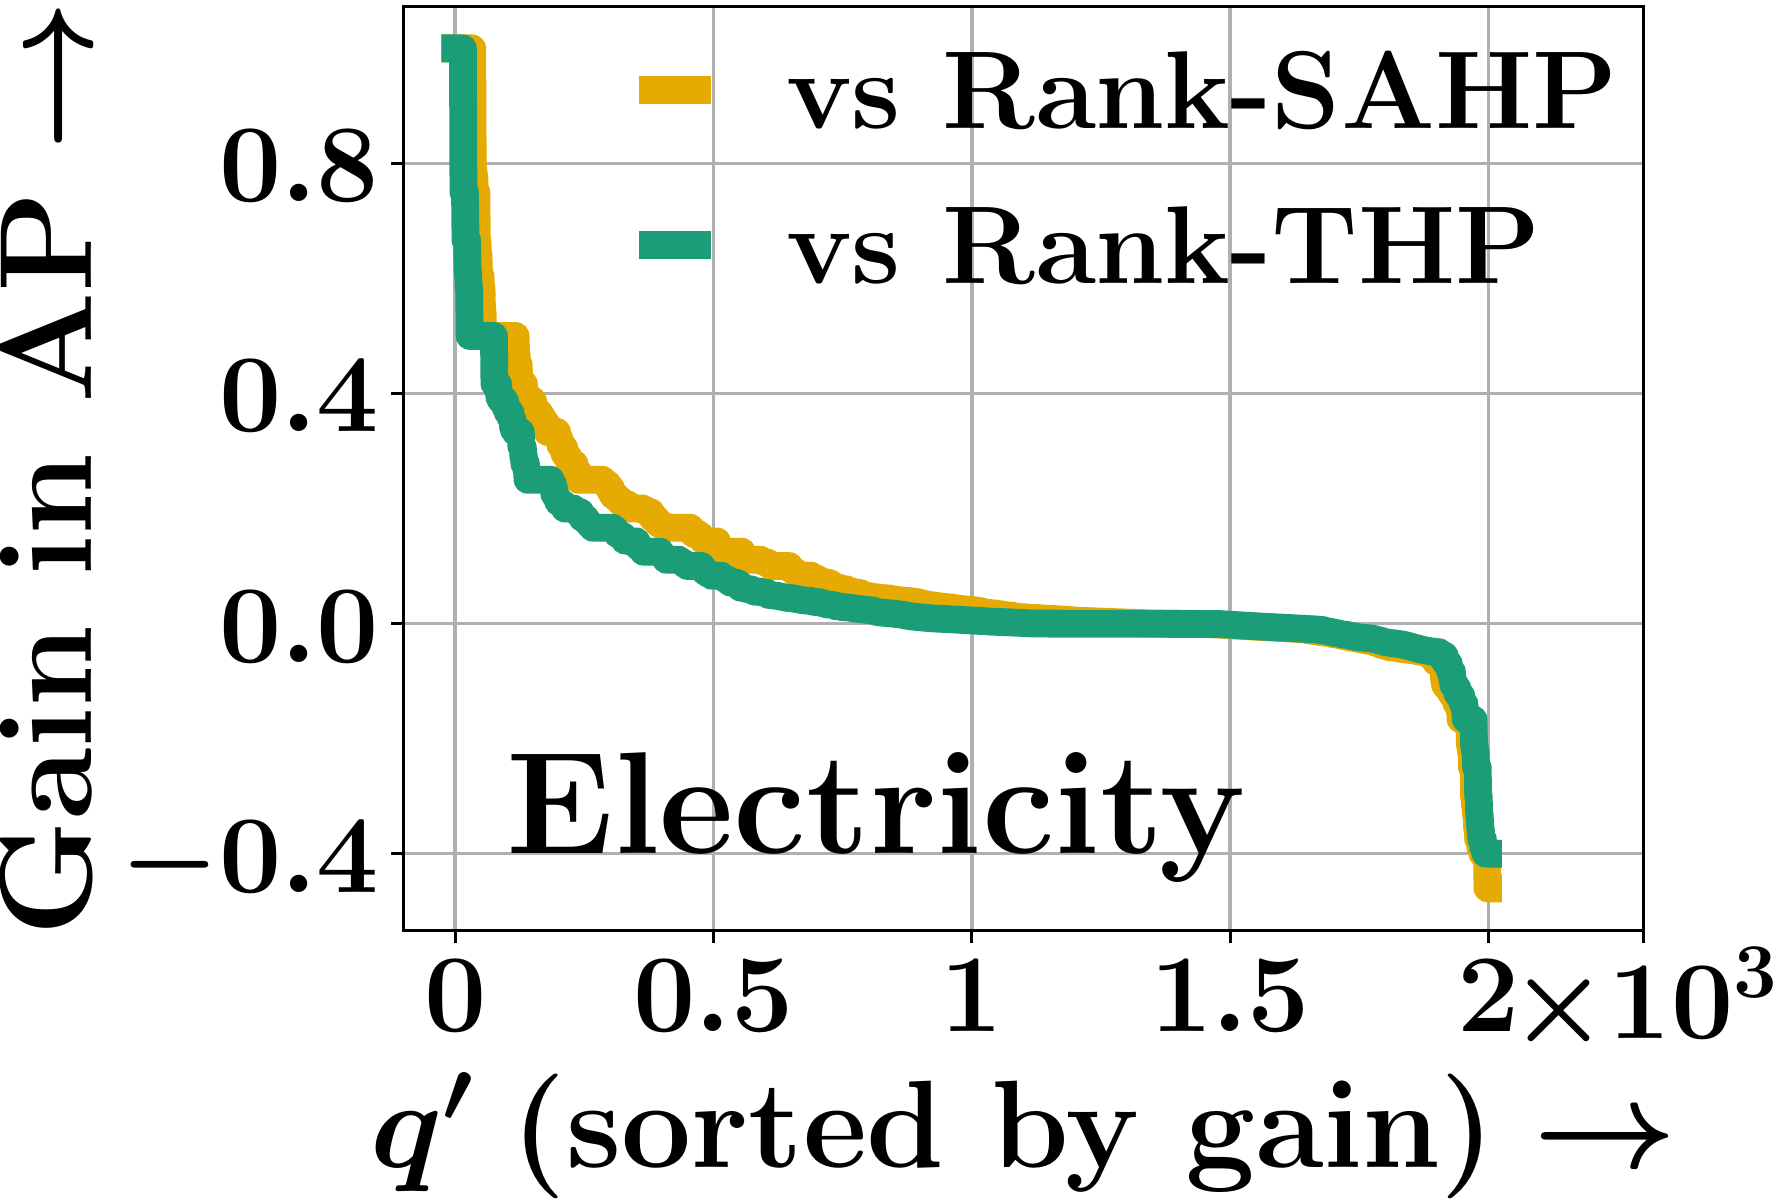}}
{\includegraphics[height=2.2cm]{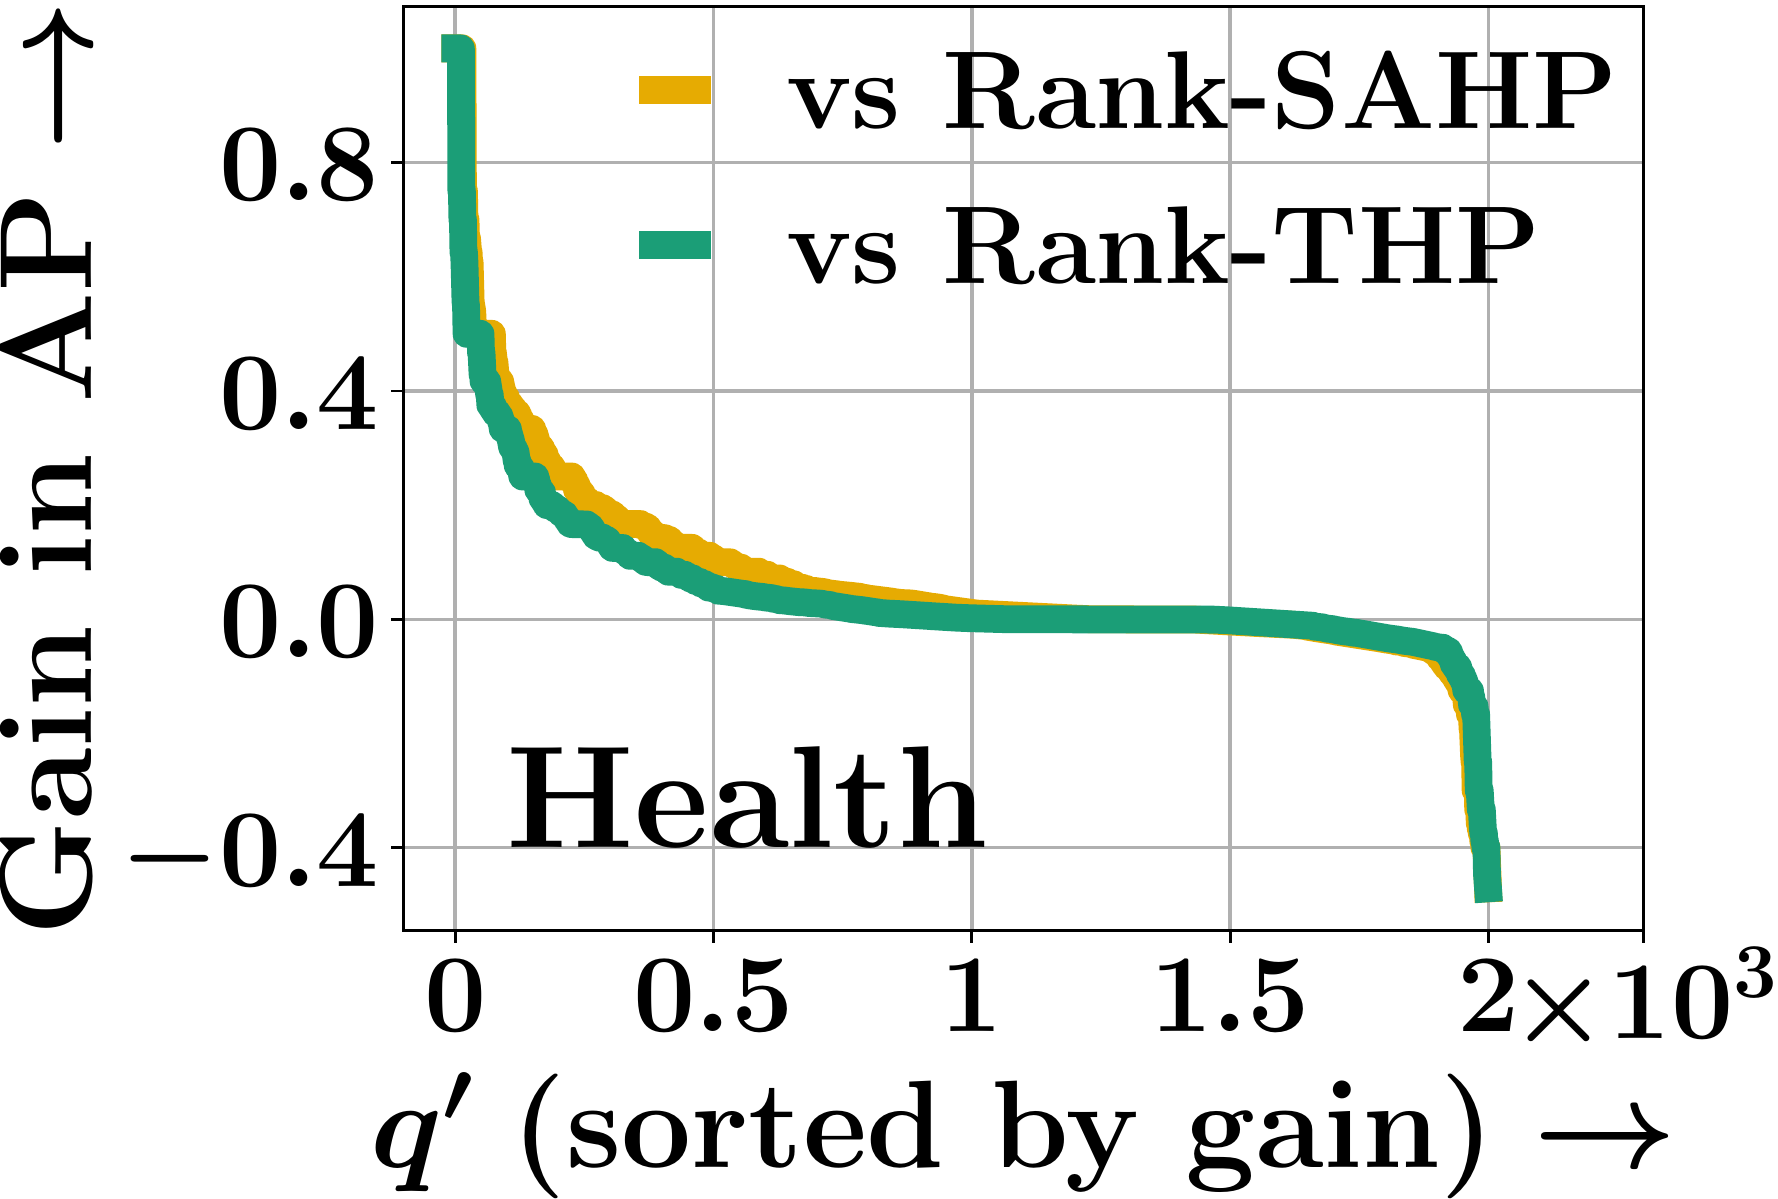}}
{\includegraphics[height=2.2cm]{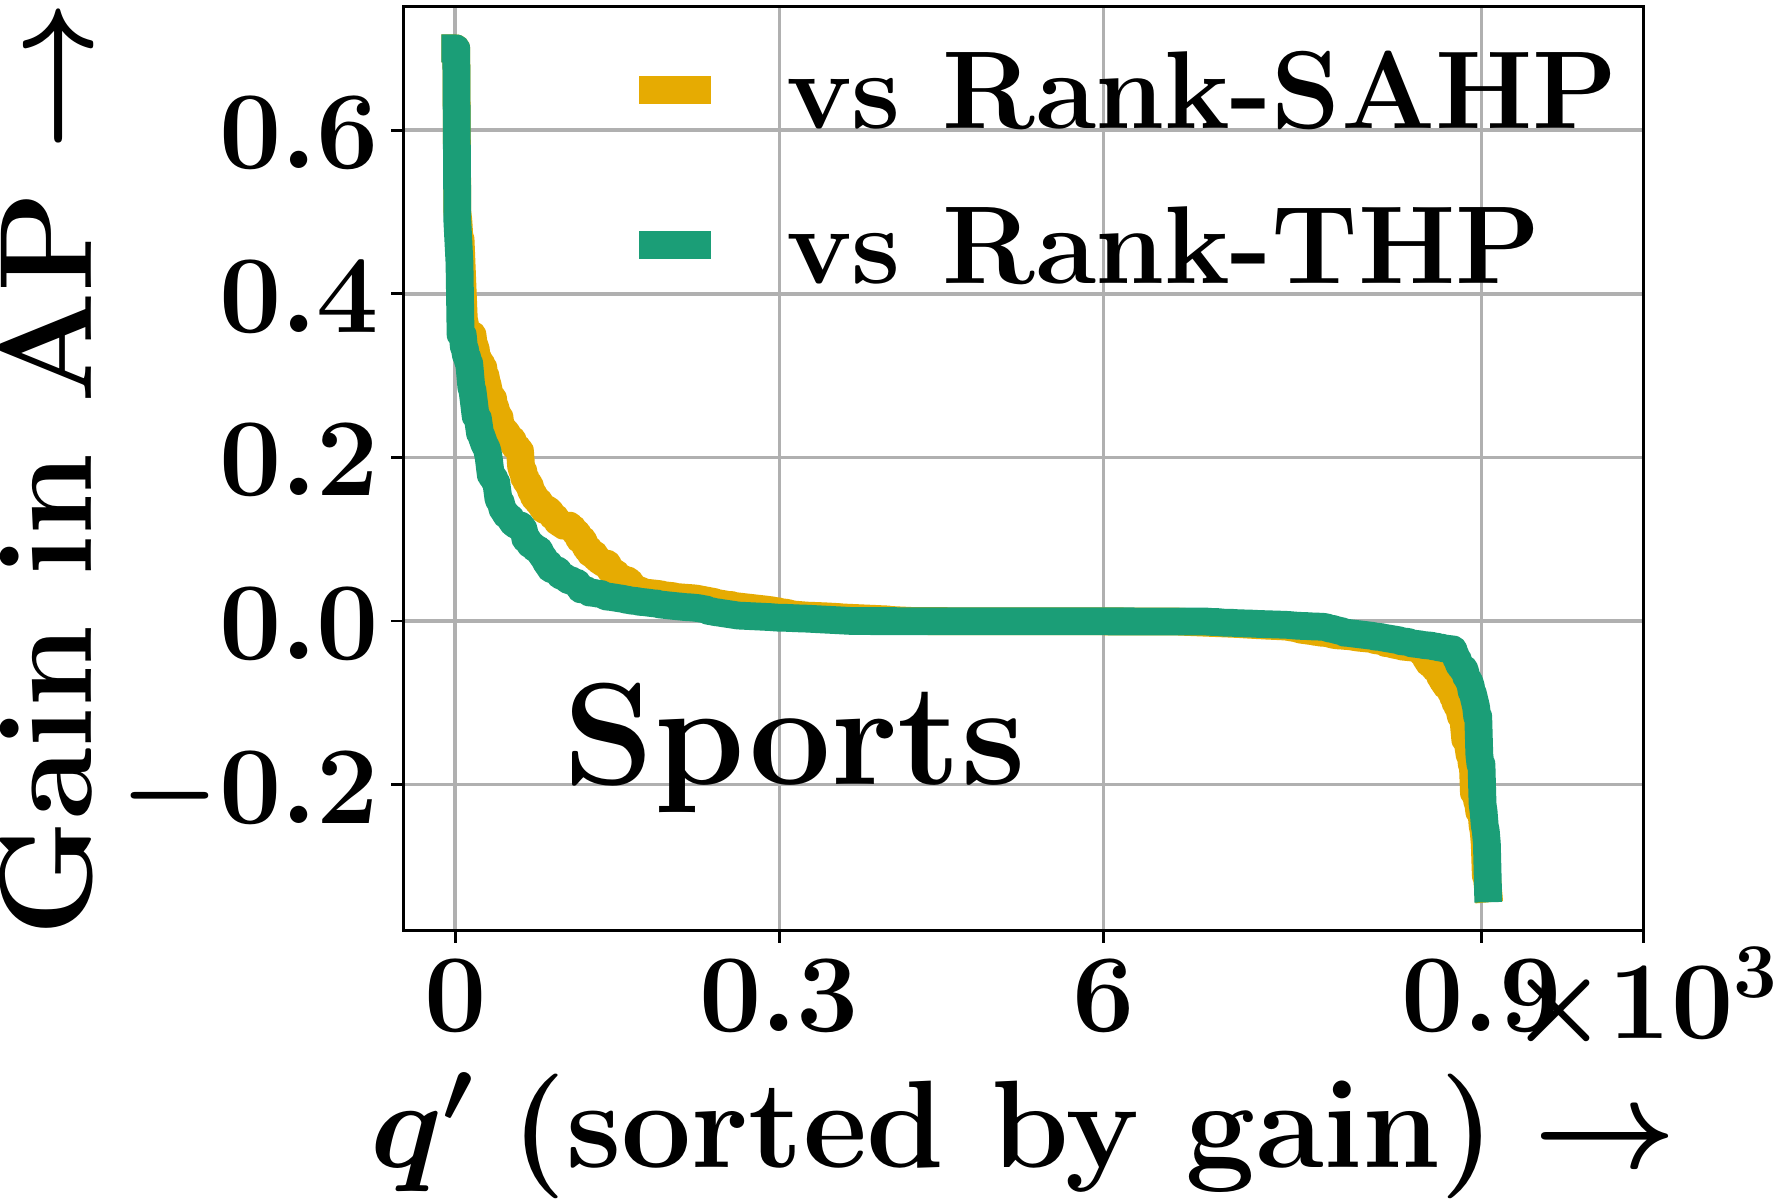}}
\caption{Query-wise performance comparison between \our and best baseline methods -- \tpprank-THP, \tpprank-SAHP. Queries are sorted by the decreasing gain in AP.}
\label{fig:app_drill}
\end{figure}

\begin{table}[t!]
	\small
	\centering
	\resizebox{0.67\textwidth}{!}{
	\begin{tabular}{l|cc}
	\toprule
	\textbf{Variant} & \textbf{Electricity} & \textbf{Sports}\\ \hline
	(i) $s_{p_{\theta},U_{\phi}} (\Hcal_q,\Hcal_c) = -\Delta_x (\Hcal_q,\Hcal_c) - \Delta_t (U_{\phi}(\Hcal_q),\Hcal_c)$ & 18.9$\pm$0.0 & 41.3$\pm$0.0\\
	(ii) $s_{p_{\theta},U_{\phi}} (\Hcal_q,\Hcal_c)= \kernel_{p_{\theta}}(\Hcal_q,\Hcal_c)$ & 30.6$\pm$0.9 & 56.3$\pm$2.1\\
	(iii) $s_{p_{\theta},U_{\phi}} (\Hcal_q,\Hcal_c)= \kernel_{p_{\theta}}(\Hcal_q,\Hcal_c) -\gamma \Delta_x (\Hcal_q,\Hcal_c)$ & 30.8$\pm$0.8 & 55.6$\pm$2.0\\
	(iv)	$s_{p_{\theta},U_{\phi}} (\Hcal_q,\Hcal_c)= \kernel_{p_{\theta}}(\Hcal_q,\Hcal_c) -\gamma \Delta_t (U_{\phi}(\Hcal_q),\Hcal_c)$ & 31.3$\pm$0.8 & 58.1$\pm$2.0\\
	(v) \ours Without $U_{\phi}(\cdot)$ & 29.7$\pm$1.3 & 56.2$\pm$2.3\\
	(vi) \ours & 32.4$\pm$0.8 & 58.7$\pm$2.1\\
	\bottomrule
	\end{tabular}
	}\\[-1.5ex]
	\caption{Ablation study of \ours and its variants in terms of MAP (in \%).}
	\label{tab:ablation_app}
\end{table}

\subsection{Ablation Study}
We also perform an ablation study for Electricity and Sports datasets in Table~\ref{tab:ablation_app}, which reveal similar insights as in Table~\ref{tab:model_ablation},

\subsection{Comparison with Random Hyperplane}
We also perform an ablation study of our efficient retrieval method along with its comparison against RH for Electricity and Sports datasets. The results in Figure.~\ref{fig:ablation_hash}, reveal similar insights as in Figure~\ref{fig:hash}.

\begin{table}[t!]
	\centering
	\begin{tabular}{|c||c|c|c|c|c|}
	\hline
	\textbf{Run Time} & \textbf{Audio} & \textbf{Celebrity} & \textbf{Electricity} & \textbf{Health} & \textbf{Sports}\\ \hline \hline
	\our & $\le$ 3hr & $\le$ 5hr & $\le$ 6hr & $\le$ 6hr & $\le$ 2hr\\ \hline
	\end{tabular}
	\caption{Training-times of \our for all datasets.}
	\label{tab:runtime}
\end{table}

\begin{figure}[t]
\centering
{\includegraphics[height=0.7cm]{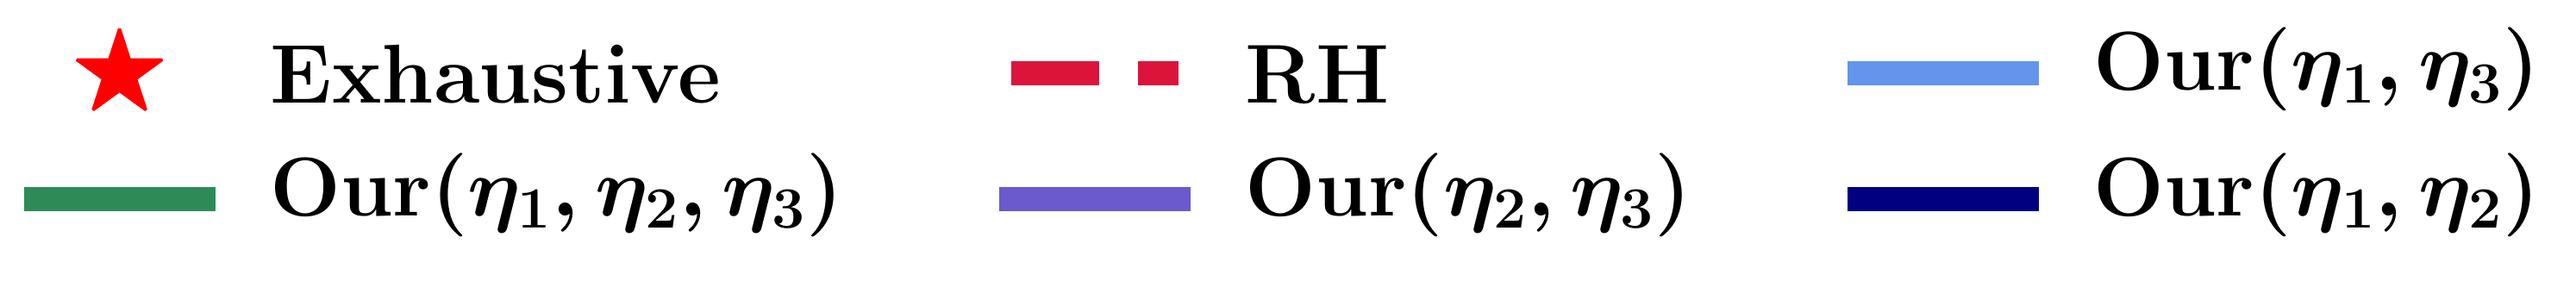}}\\
\subfloat
{\includegraphics[height=2.2cm]{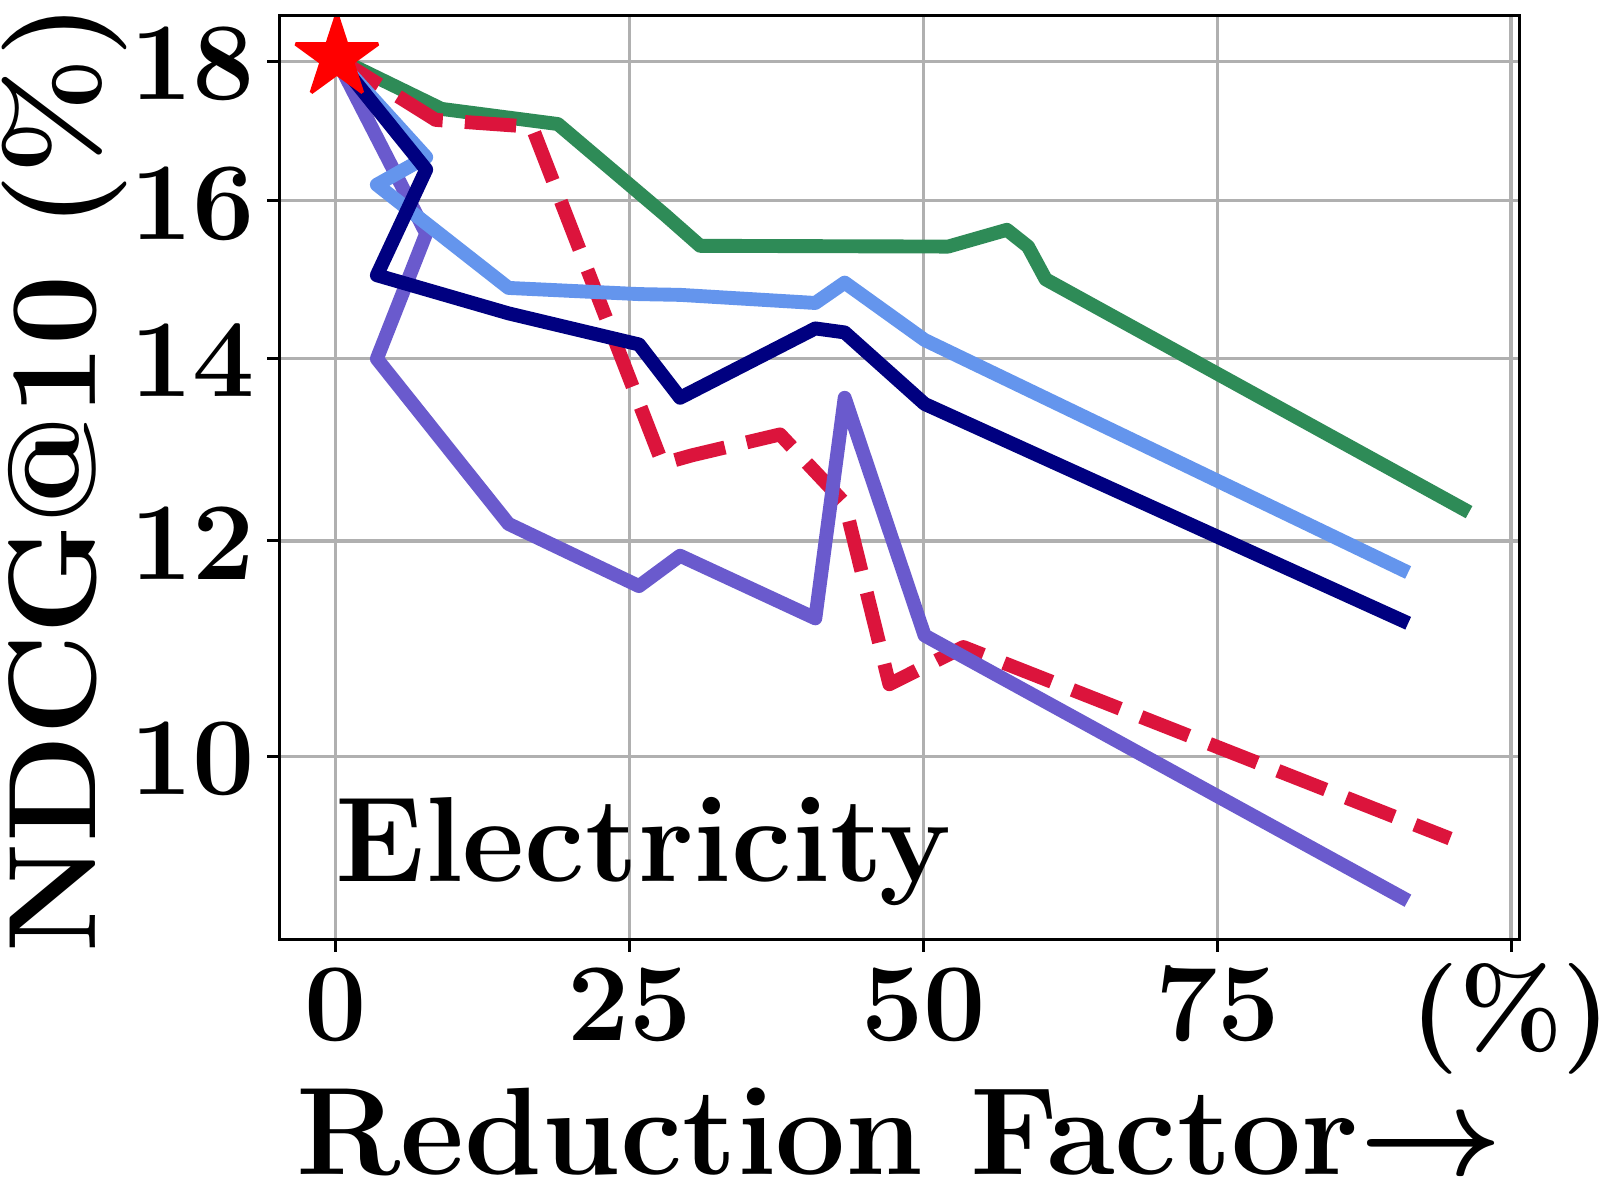}}
\hspace{0.5cm}
\subfloat
{\includegraphics[height=2.2cm]{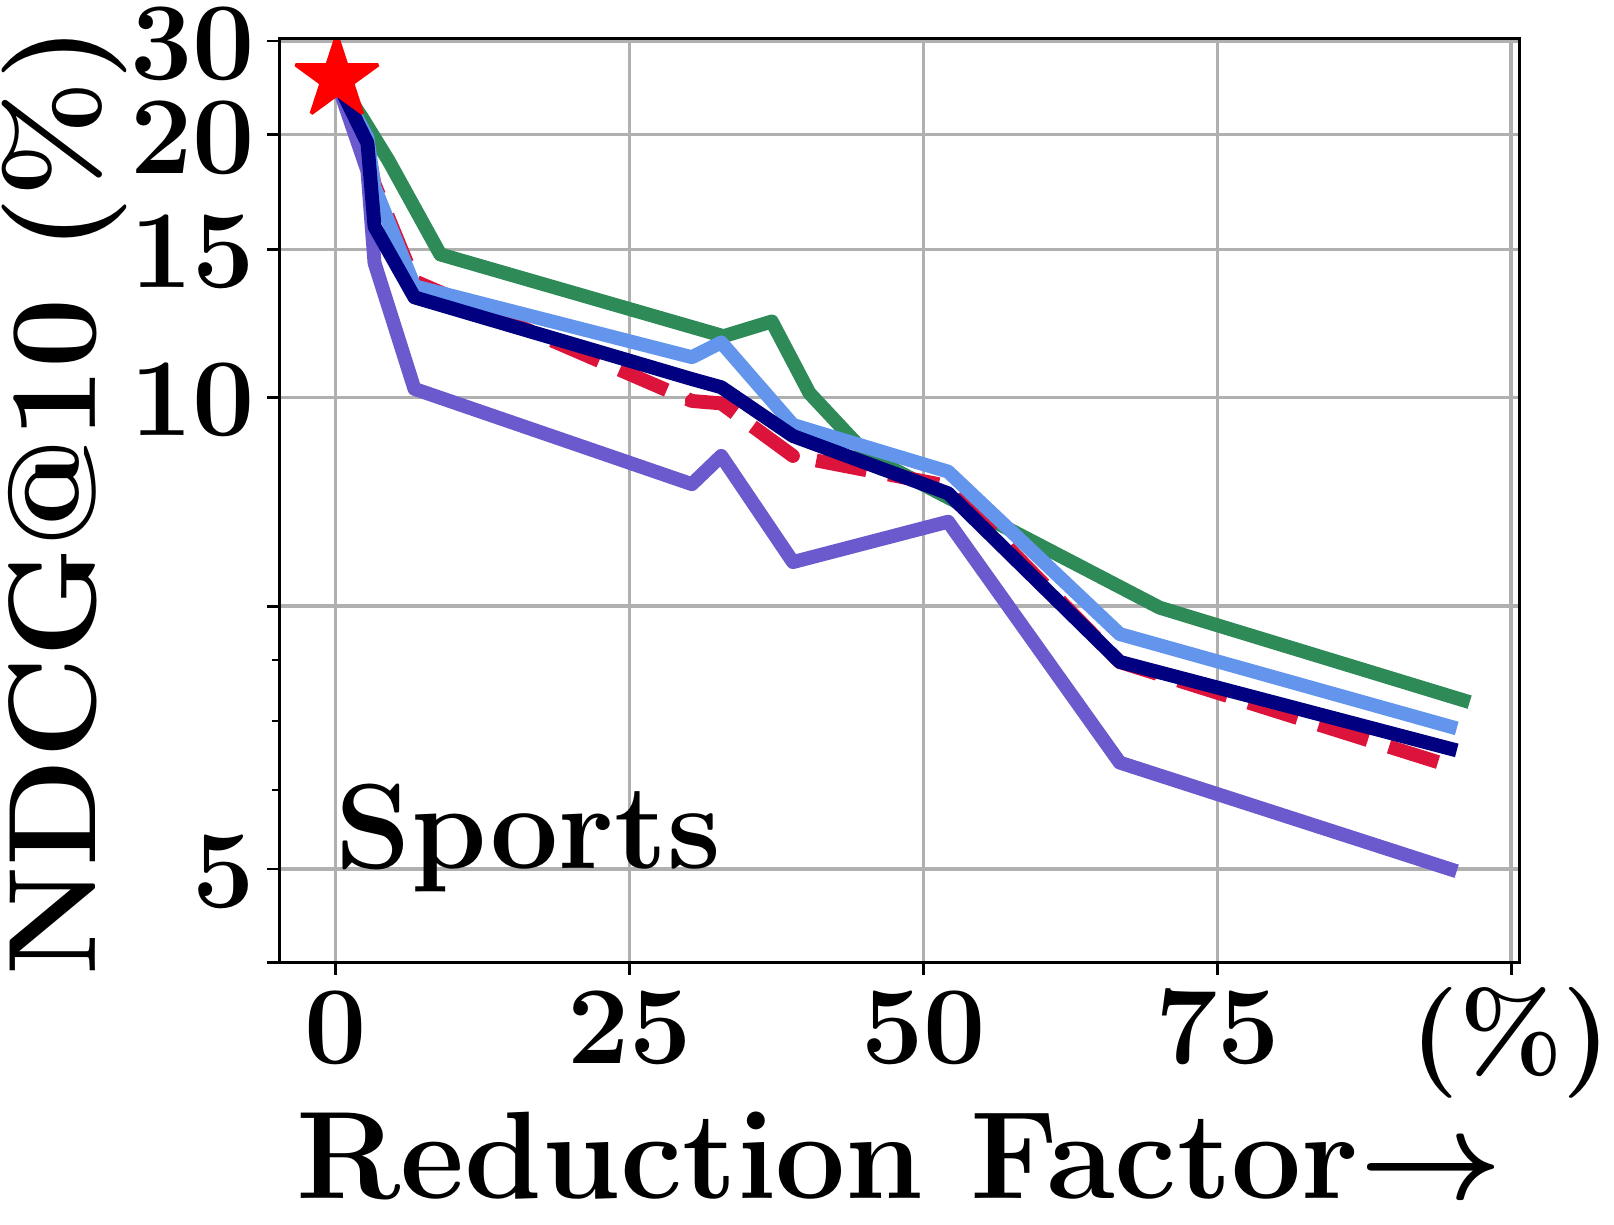}}
\caption{Tradeoff between NDCG@10 vs. Reduction factor, \ie, \% reduction in number of comparisons between query-corpus pairs w.r.t. the exhaustive comparisons for different hashing methods. The point marked as $ \color{red} {\star}$ indicates the case with exhaustive comparisons on the set of corpus sequences.}
\label{fig:ablation_hash}
\end{figure}

\begin{table}[t!]
	\small
	\centering
	\resizebox{0.6\textwidth}{!}{
	\begin{tabular}{l|ccccc}
	\hline
	\textbf{$|\mathcal{H}_q| = (10,20)$} & \textbf{Audio} & \textbf{Celebrity} & \textbf{Health} & \textbf{Electricity} & \textbf{Sports}\\ \hline
	\texttt{Rank}-THP & 18.97 & 22.06 & 9.48 & 12.27 & 26.58\\
	\ours & 21.30 & 25.77 & 15.83 & 10.79 & 27.63\\
	\hline
	\end{tabular}
	}\\[-1.5ex]
	\caption{Retrieval quality in terms of mean average precision (MAP) for query sequence lengths sampled between 10 and 50.}
	\label{tab:length1}
	\centering
	\resizebox{0.6\textwidth}{!}{
	\begin{tabular}{l|ccccc}
	\hline
	\textbf{$|\mathcal{H}_q| = (50,100)$} & \textbf{Audio} & \textbf{Celebrity} & \textbf{Health} & \textbf{Electricity} & \textbf{Sports}\\ \hline
	\texttt{Rank}-THP & 27.94 & 37.85 & 17.58 & 21.61 & 31.26\\
	\ours & 28.58 & 41.92 & 19.67 & 23.54 & 36.92\\
	\hline
	\end{tabular}
	}\\[-1.5ex]
	\caption{Retrieval quality in terms of mean average precision (MAP) for query sequence lengths sampled between 50 and 100.}
	\label{tab:length2}
\end{table}

\subsection{Runtime Analysis}
Next, we calculate the run-time performance of \our. With this experiment, our goal is to determine if the training times of \our are suitable for designing solutions for real-world problems. From the results in Table~\ref{tab:runtime}, we note that even for datasets with up to 60 million events, the training times are well within the feasible range for practical deployment.

\subsection{Query Length}
We perform an additional experiment of sequence retrieval with varying query lengths. Specifically, we sample queries of lengths $|\mathcal{H}_q| \sim Unif(10, 50)$ and $|\mathcal{H}_q| \sim Unif(50, 100)$ and report the sequence retrieval results in Table~\ref{tab:length1} and Table ~\ref{tab:length2} respectively. The results show that the performance of all models deteriorates significantly as we reduce the length of query sequences. They also show that even with smaller query lengths, \ours significantly outperforms the other state-of-the-art baseline \texttt{Rank}-THP.

\subsection{Qualitative Analysis}
To get deeper insights into the working of our model, we perform a qualitative analysis between a query sequence from the dataset and the sequence retrieved by \our. More specifically, we aim to understand the similar patterns between query and corpus sequences that \our searches for in the corpus and plot the query sequence and the corresponding top-ranked relevant corpus sequence retrieved by \our. The results across all datasets in Figure~\ref{fig:qualitative} show that the inter-arrival times of the CTES retrieved by \our closely matches with the query inter-arrival times.

\begin{figure}
\centering
 \subfloat[Audio dataset]
 {\includegraphics[height=3cm]{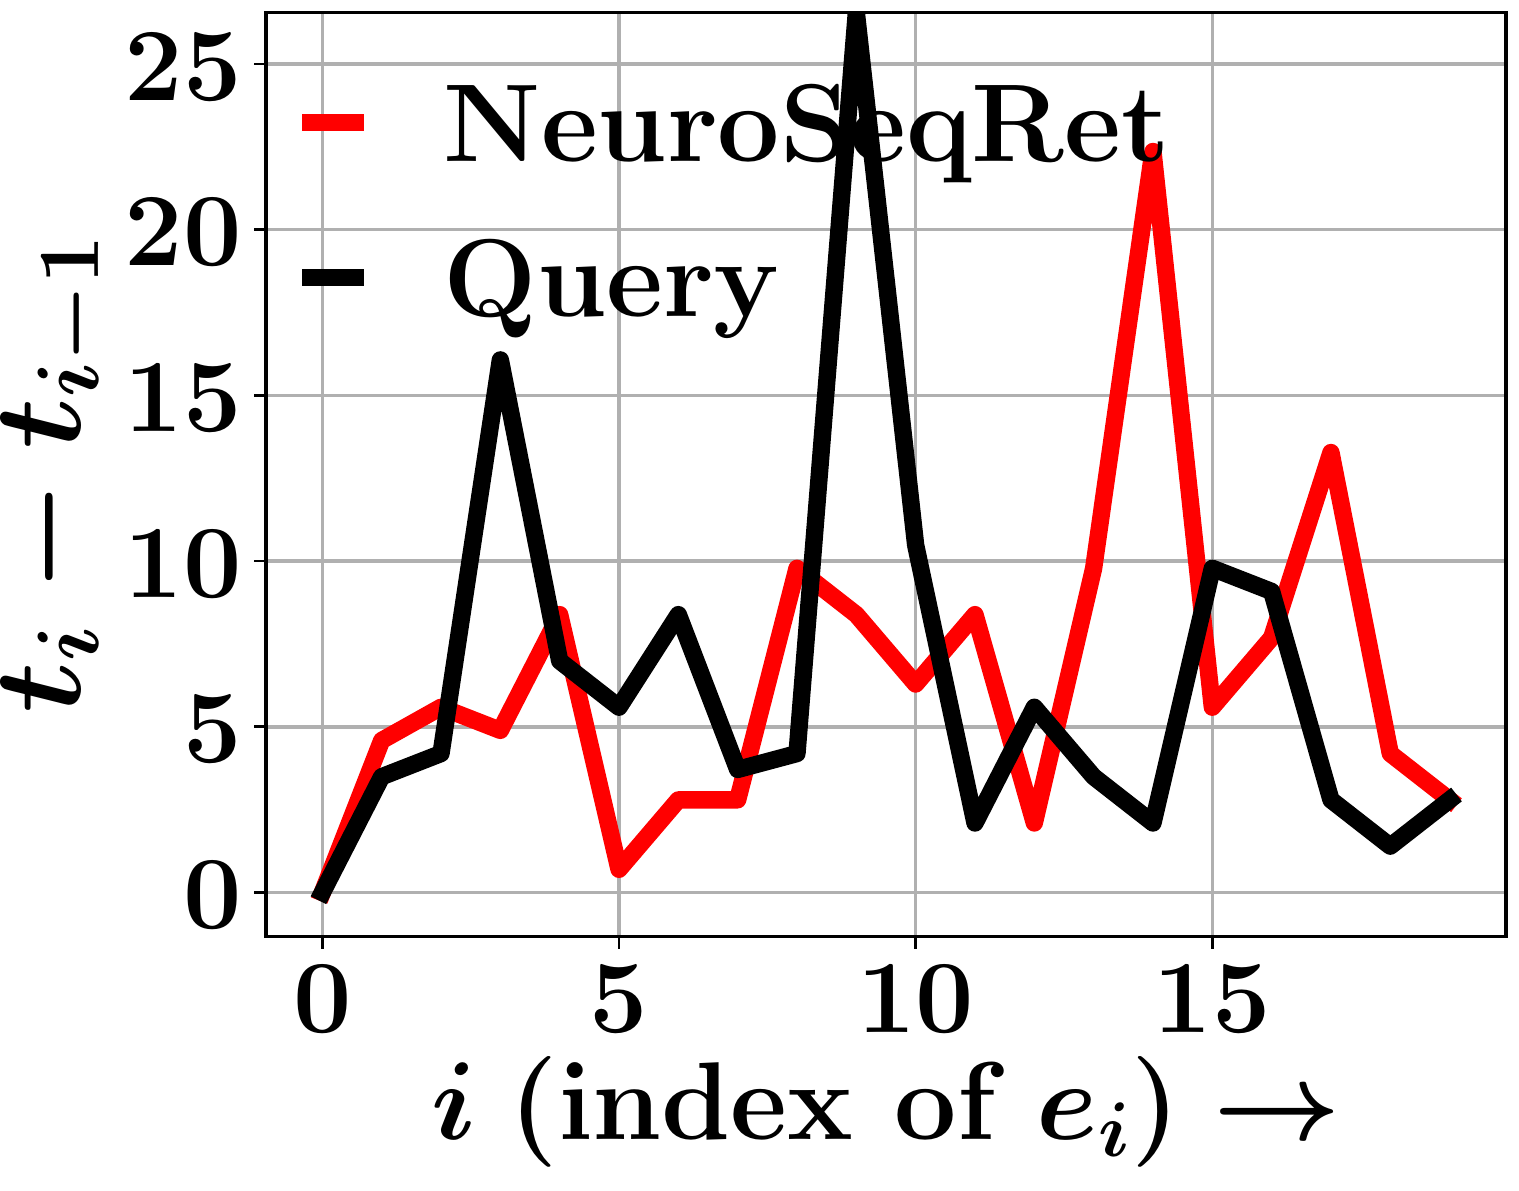}}
 {\includegraphics[height=3cm]{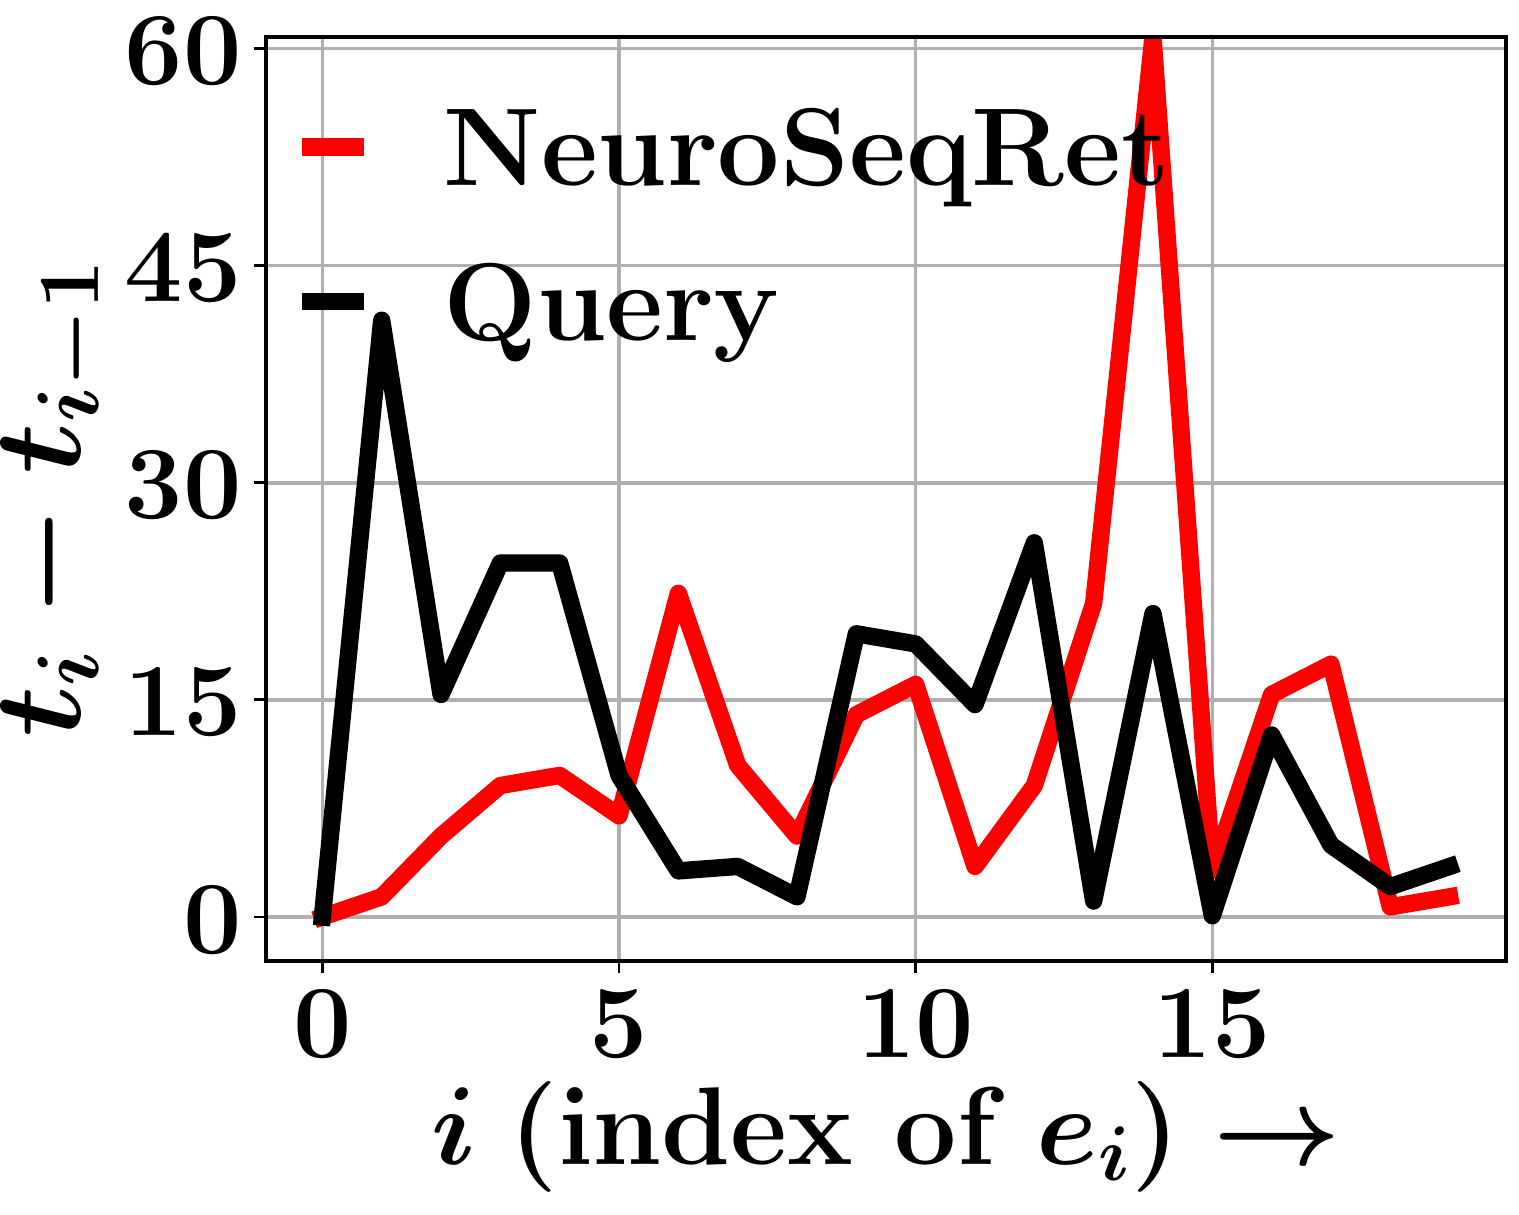}}
 {\includegraphics[height=3cm]{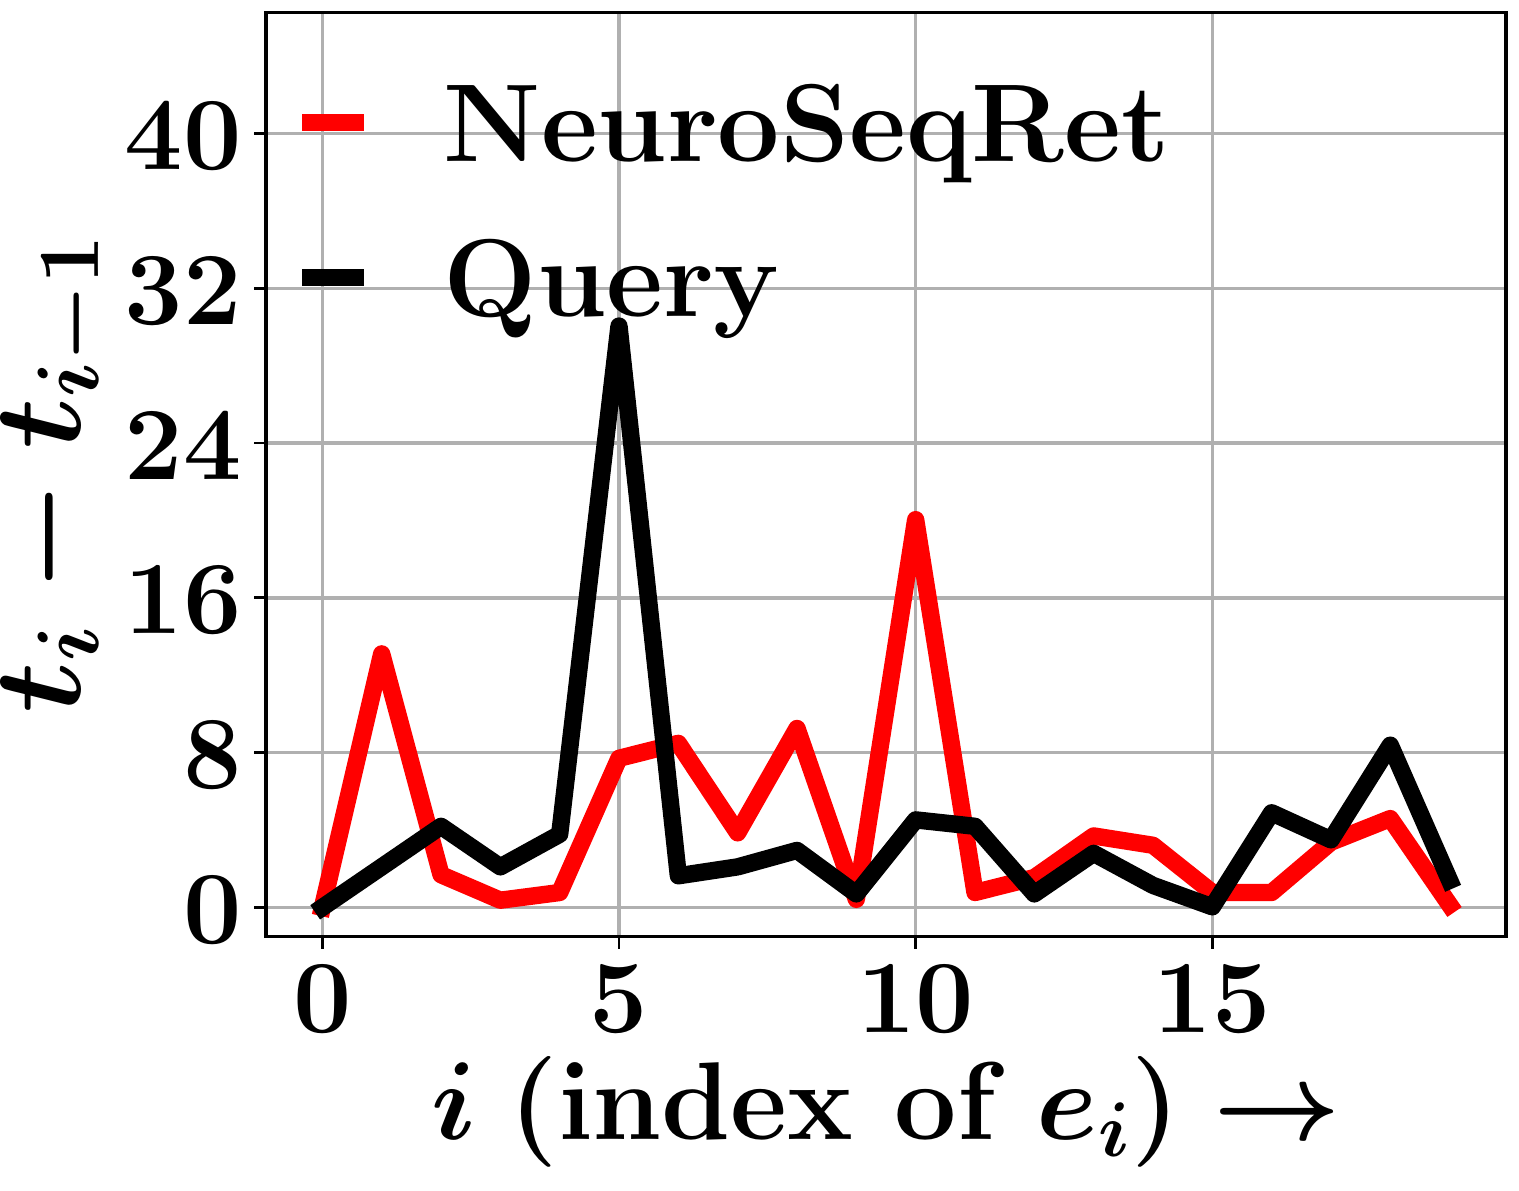}}
 {\includegraphics[height=3cm]{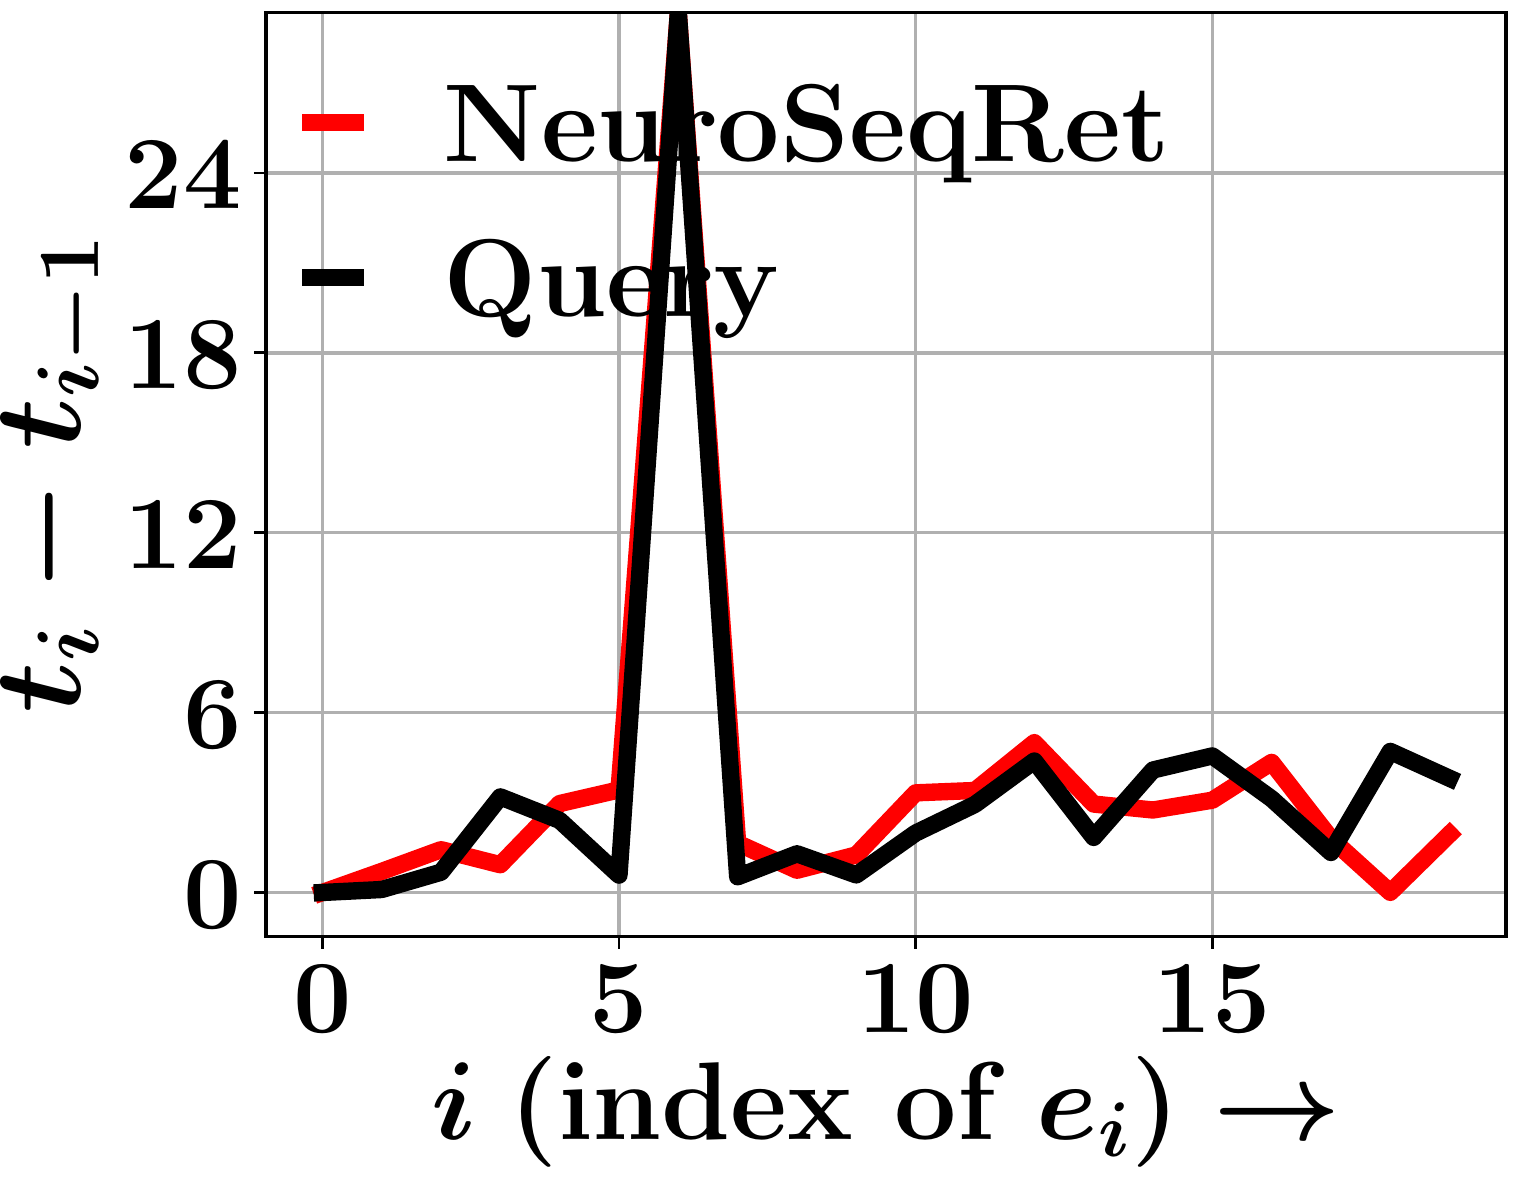}}

\subfloat[Celebrity dataset]
{\includegraphics[height=3cm]{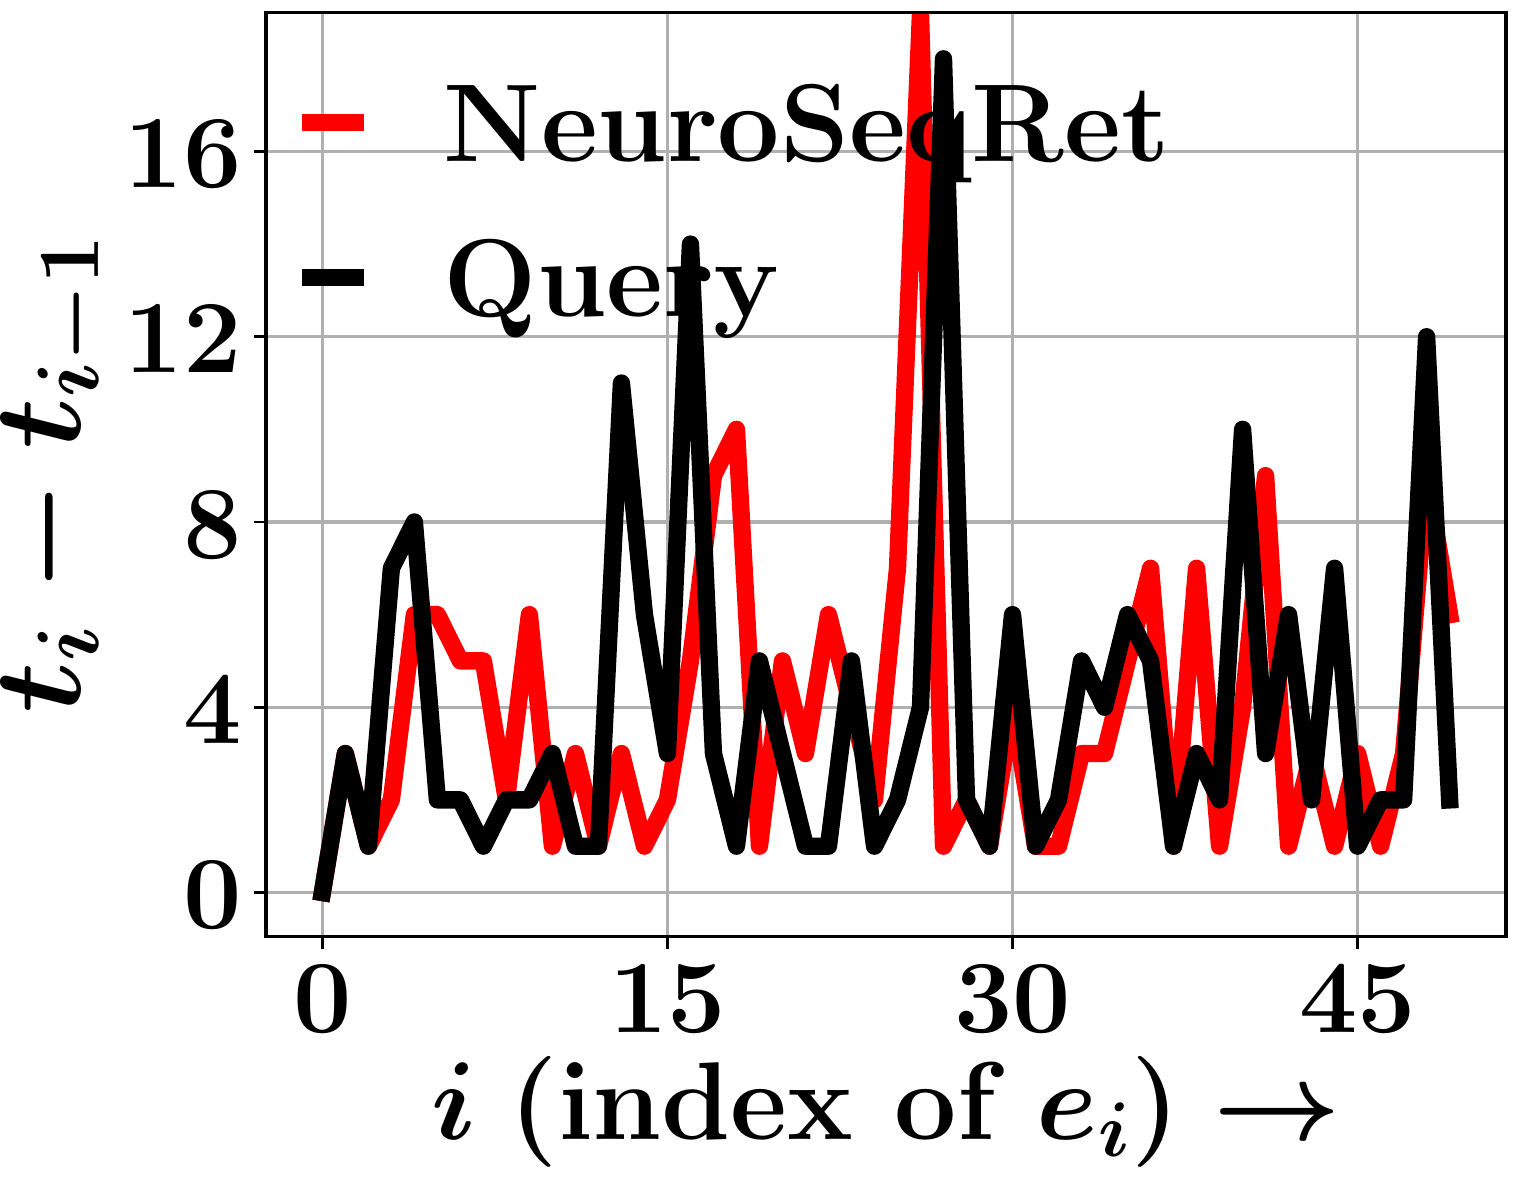}}
{\includegraphics[height=3cm]{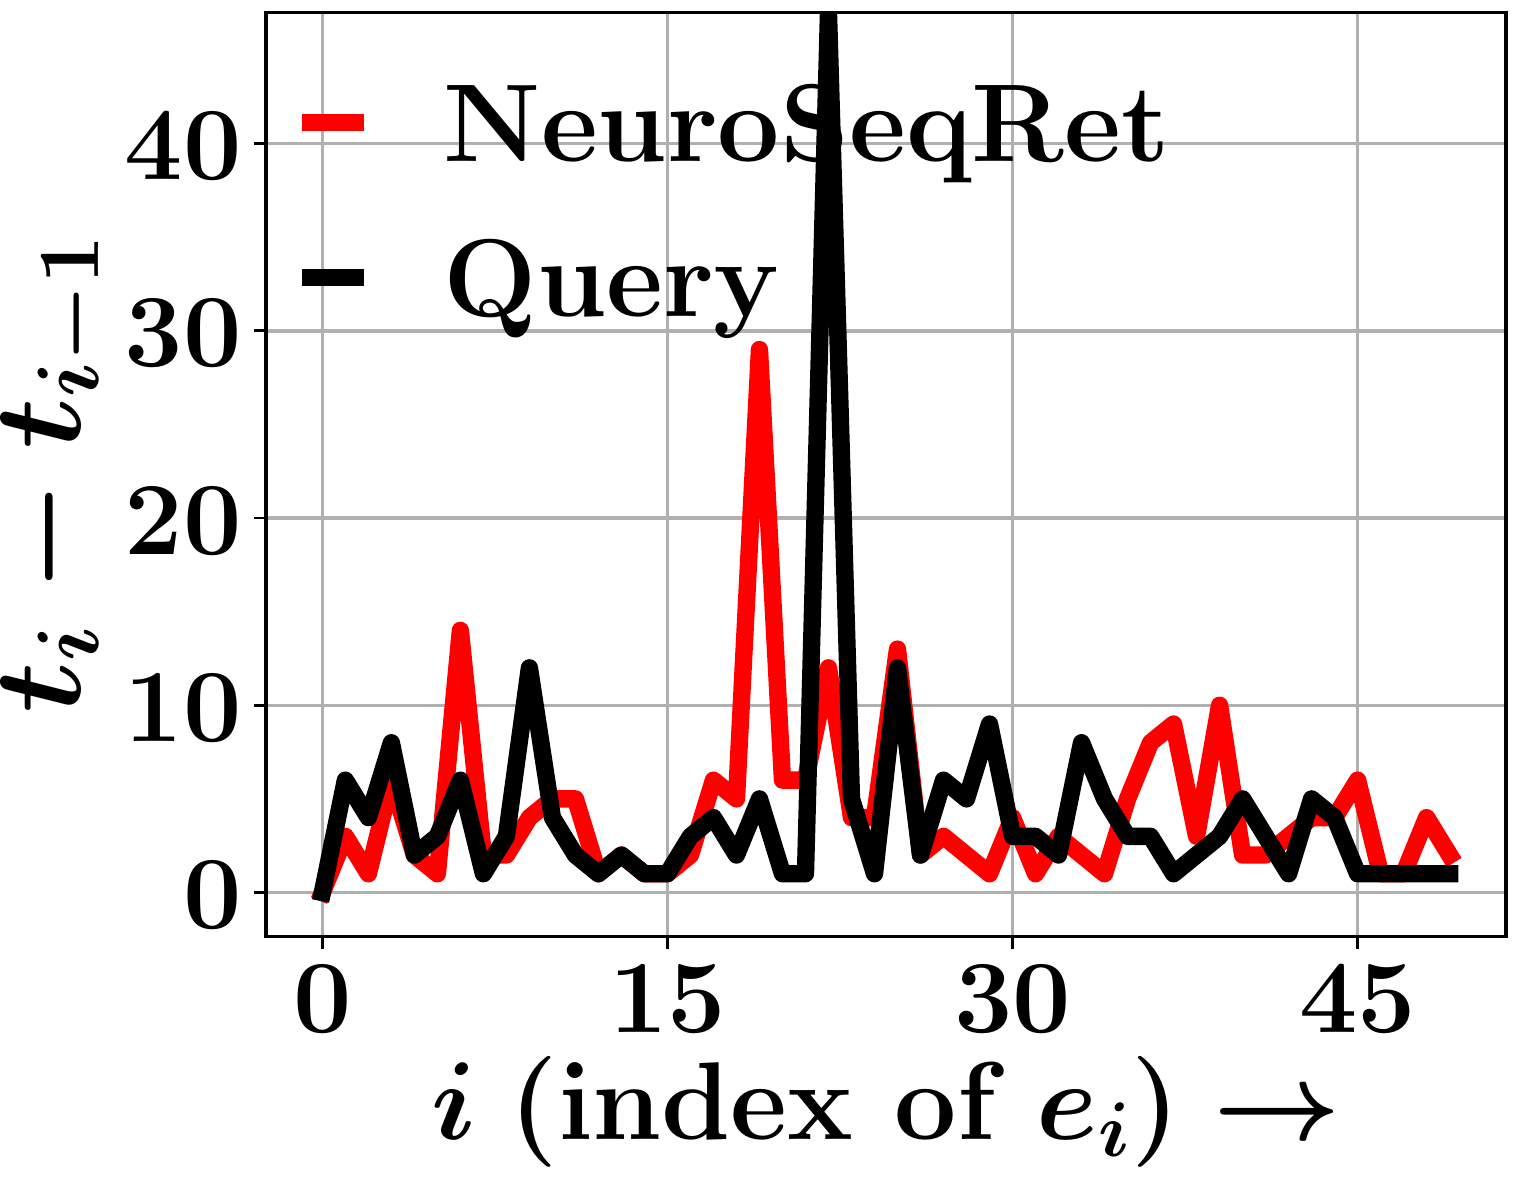}}
{\includegraphics[height=3cm]{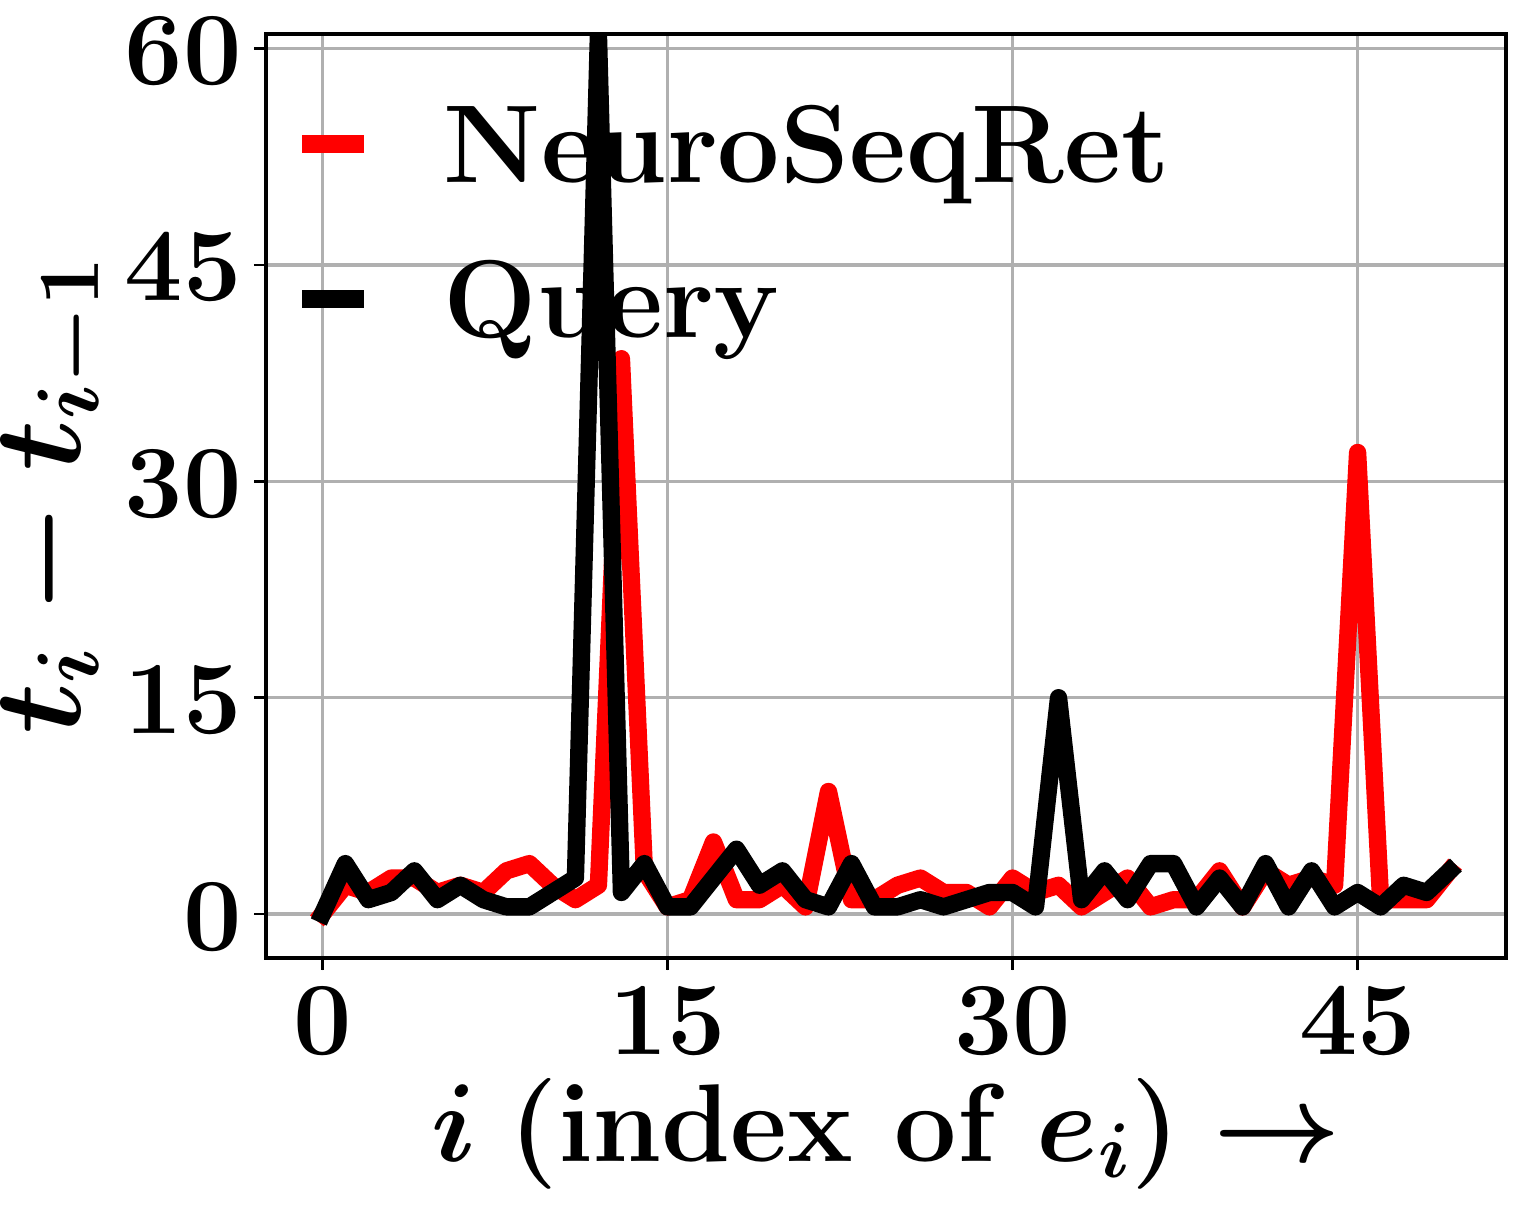}}
{\includegraphics[height=3cm]{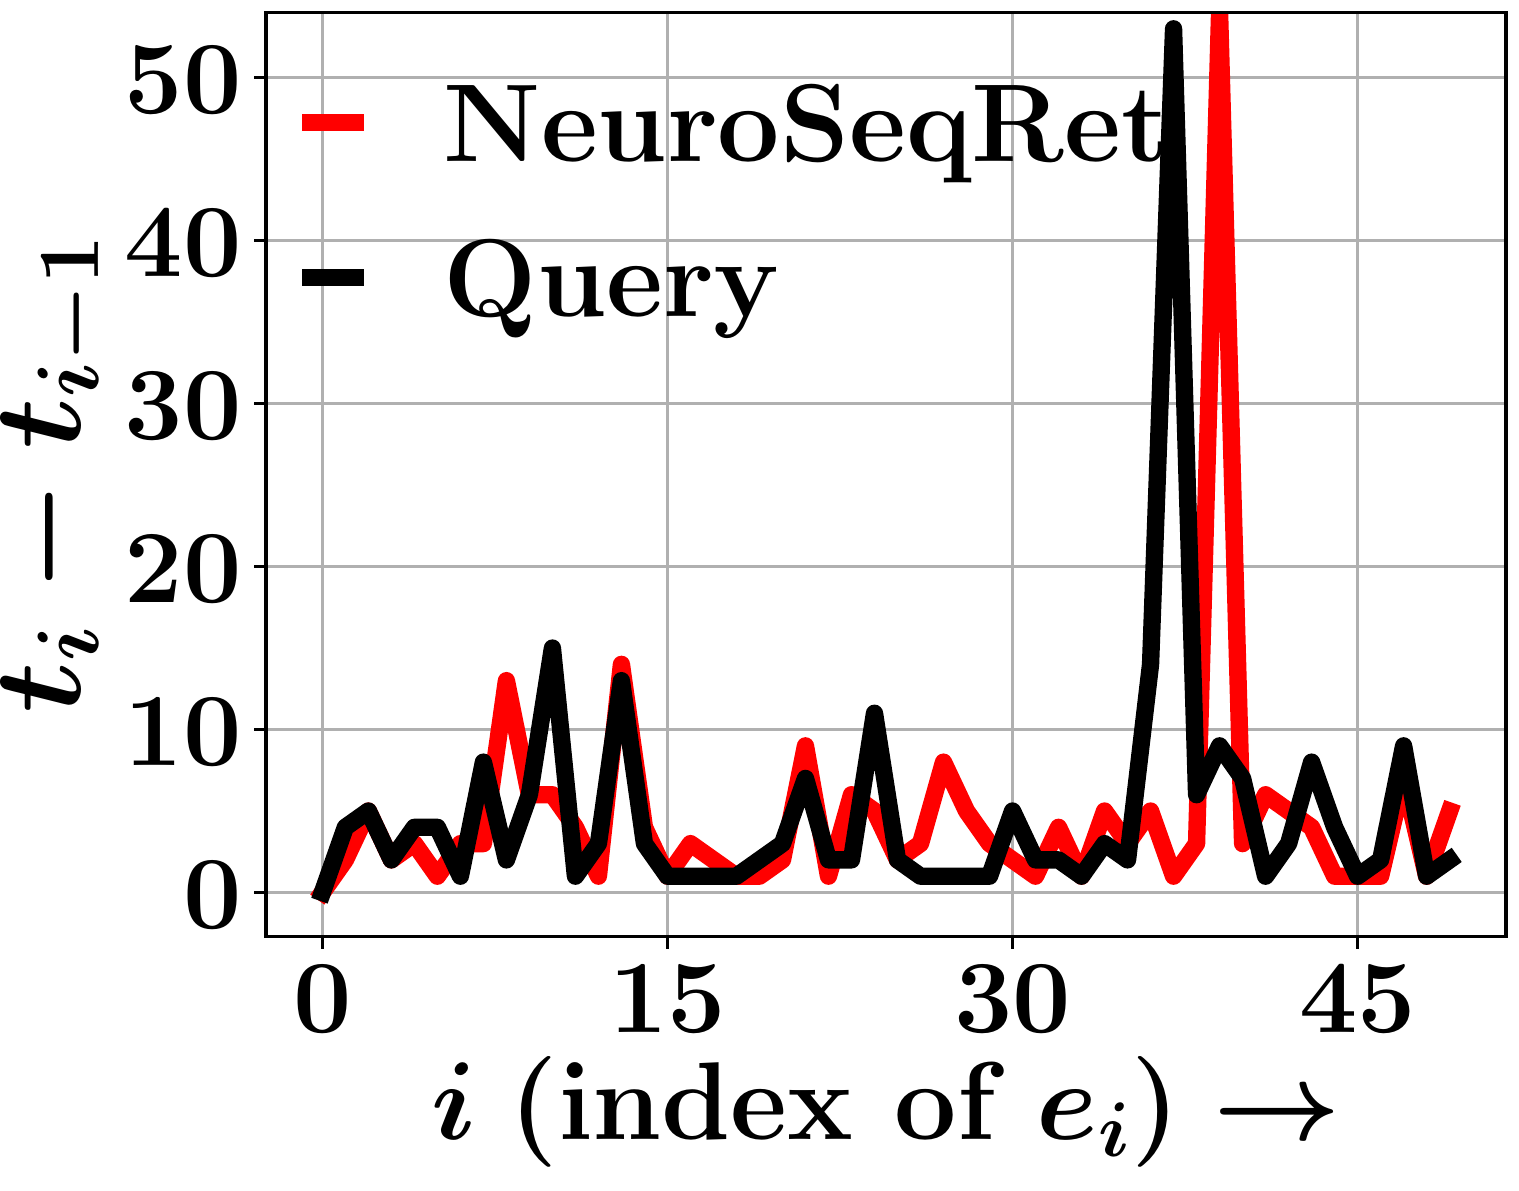}}

\subfloat[Electricity dataset]
{\includegraphics[height=3cm]{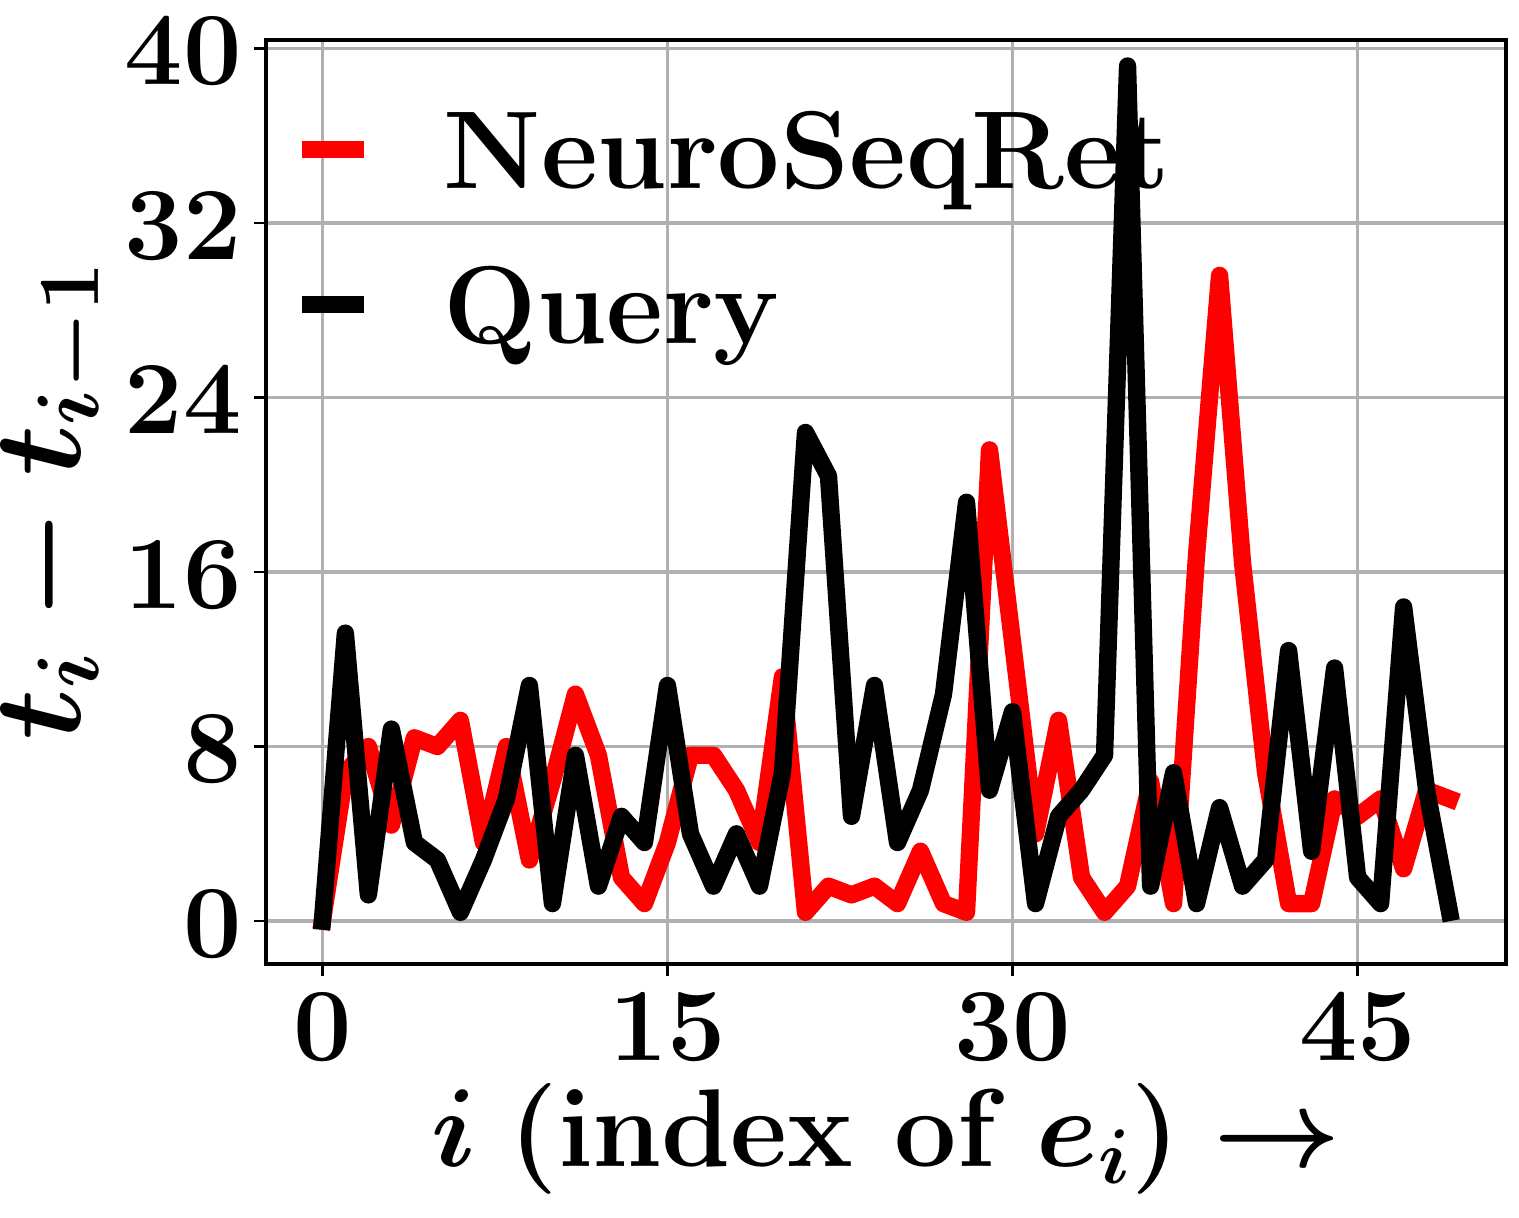}}
{\includegraphics[height=3cm]{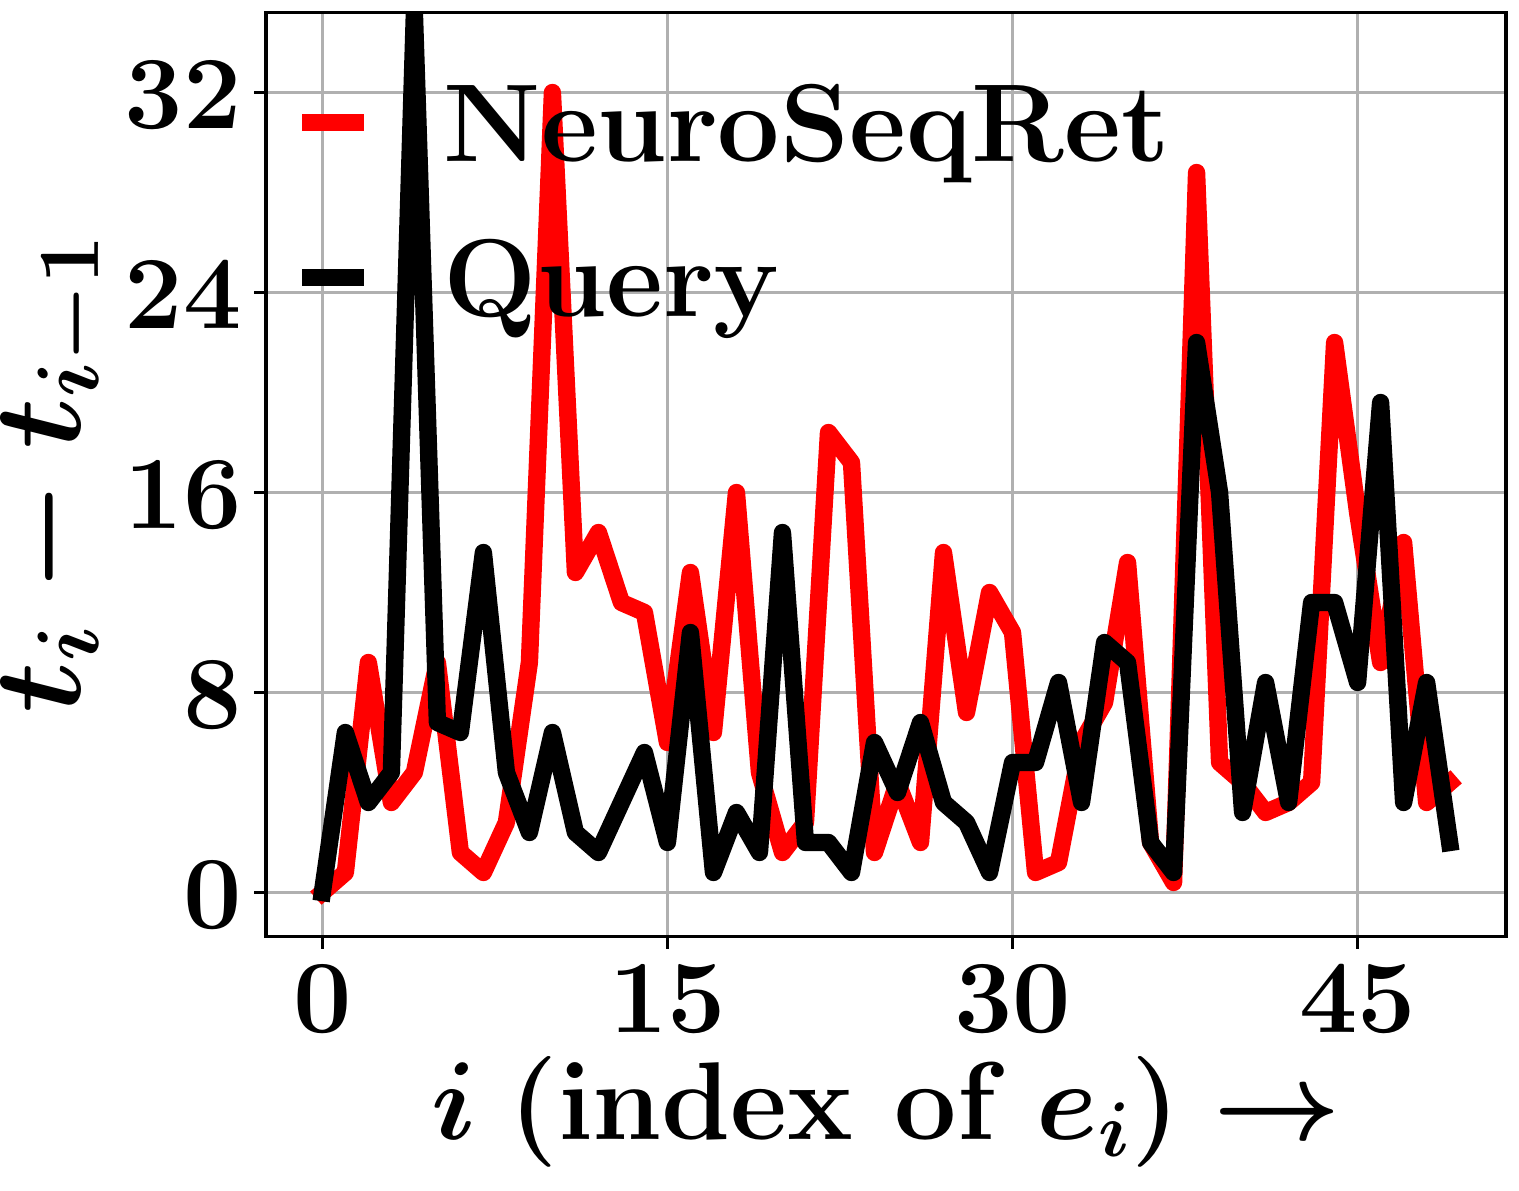}}
{\includegraphics[height=3cm]{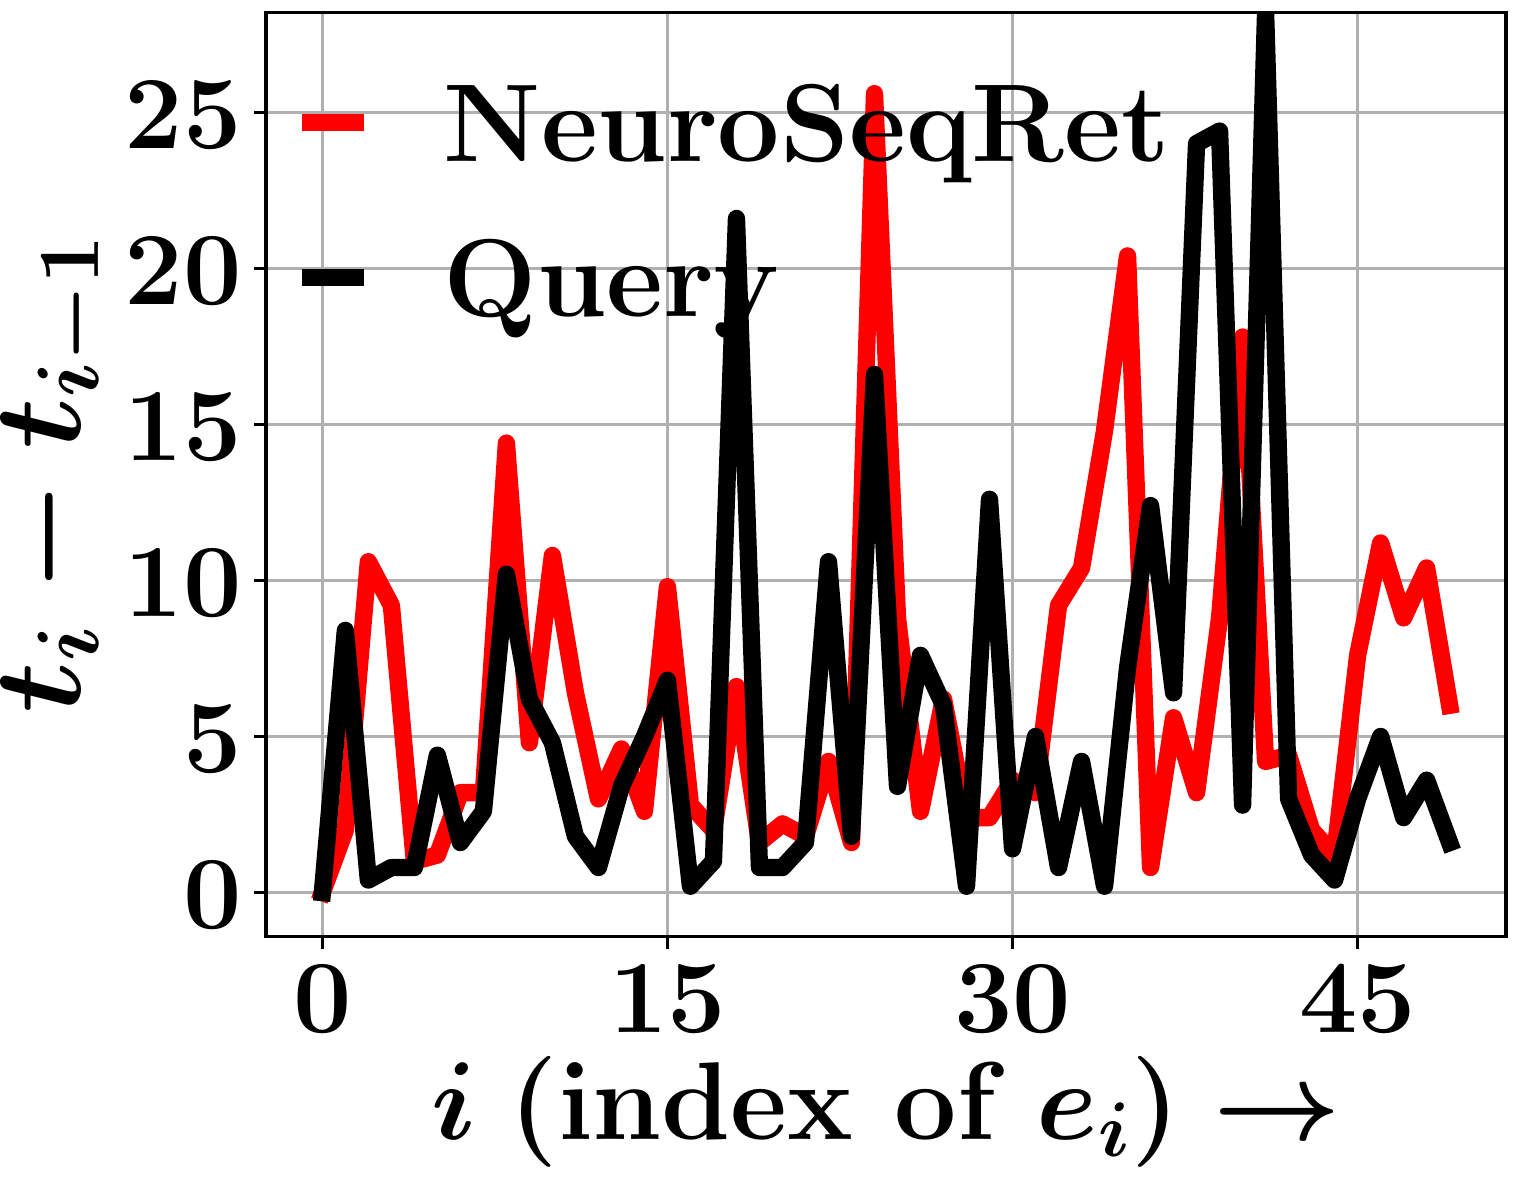}}
{\includegraphics[height=3cm]{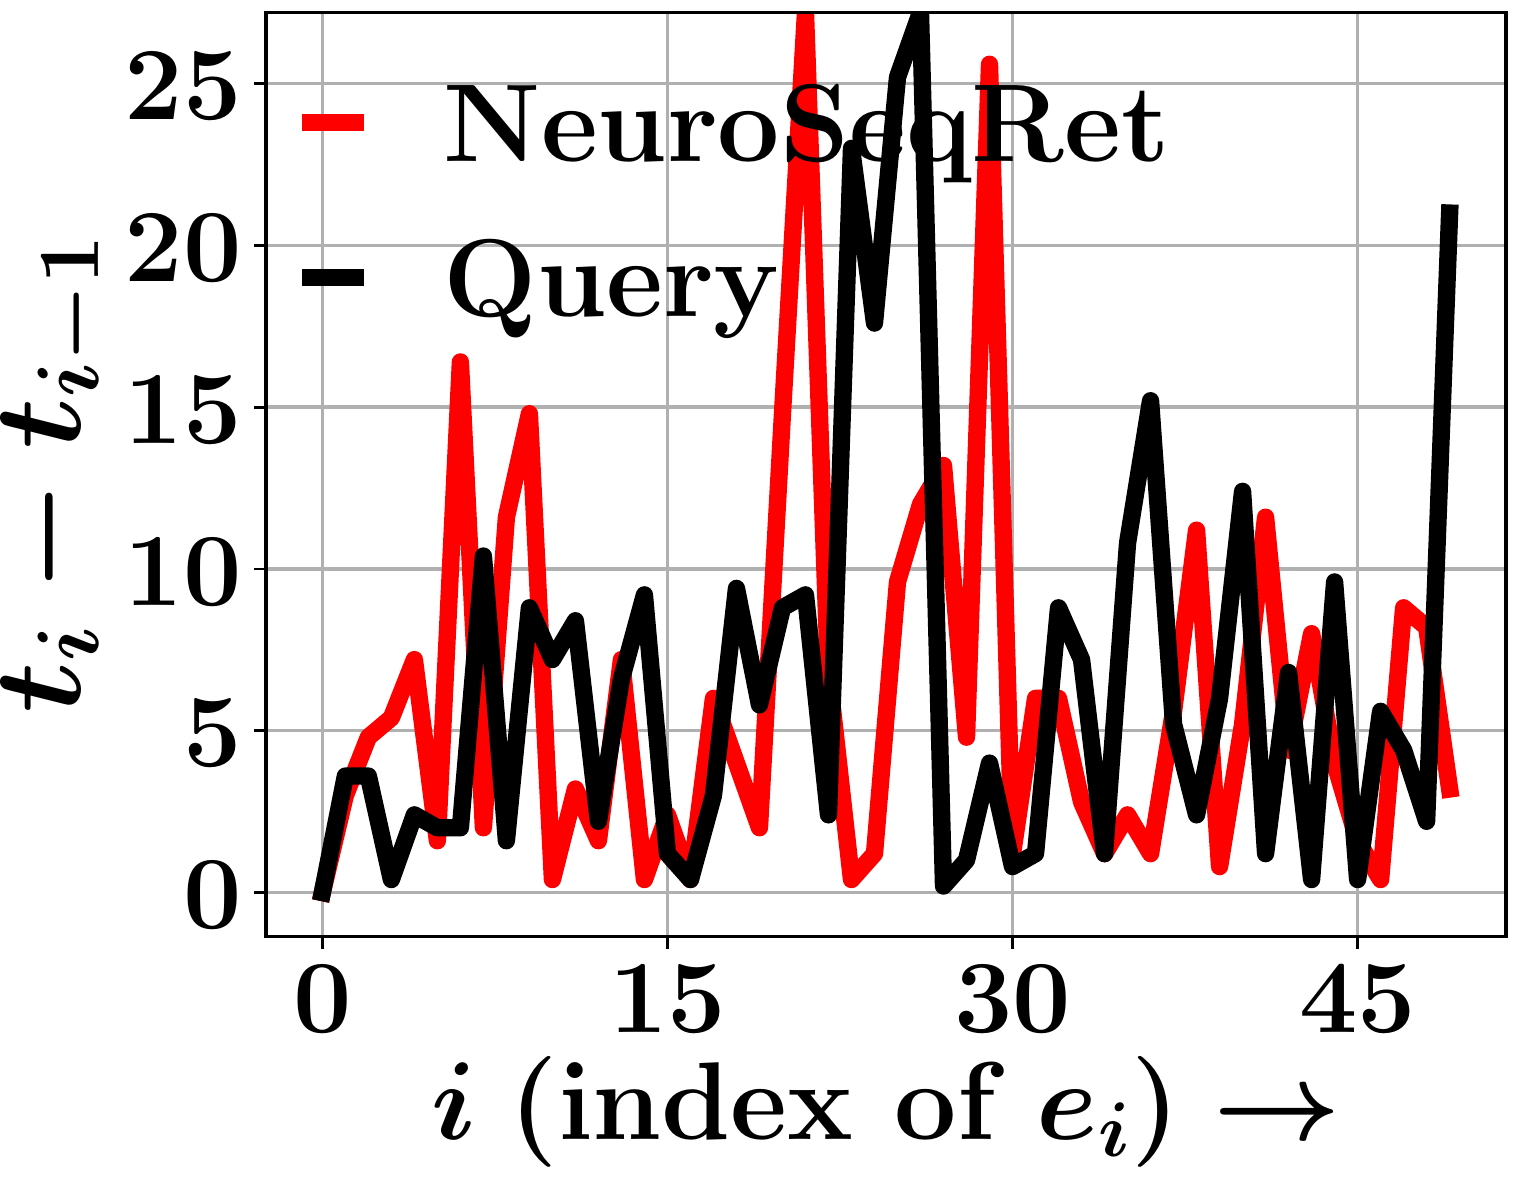}}

\subfloat[Health dataset]
{\includegraphics[height=3cm]{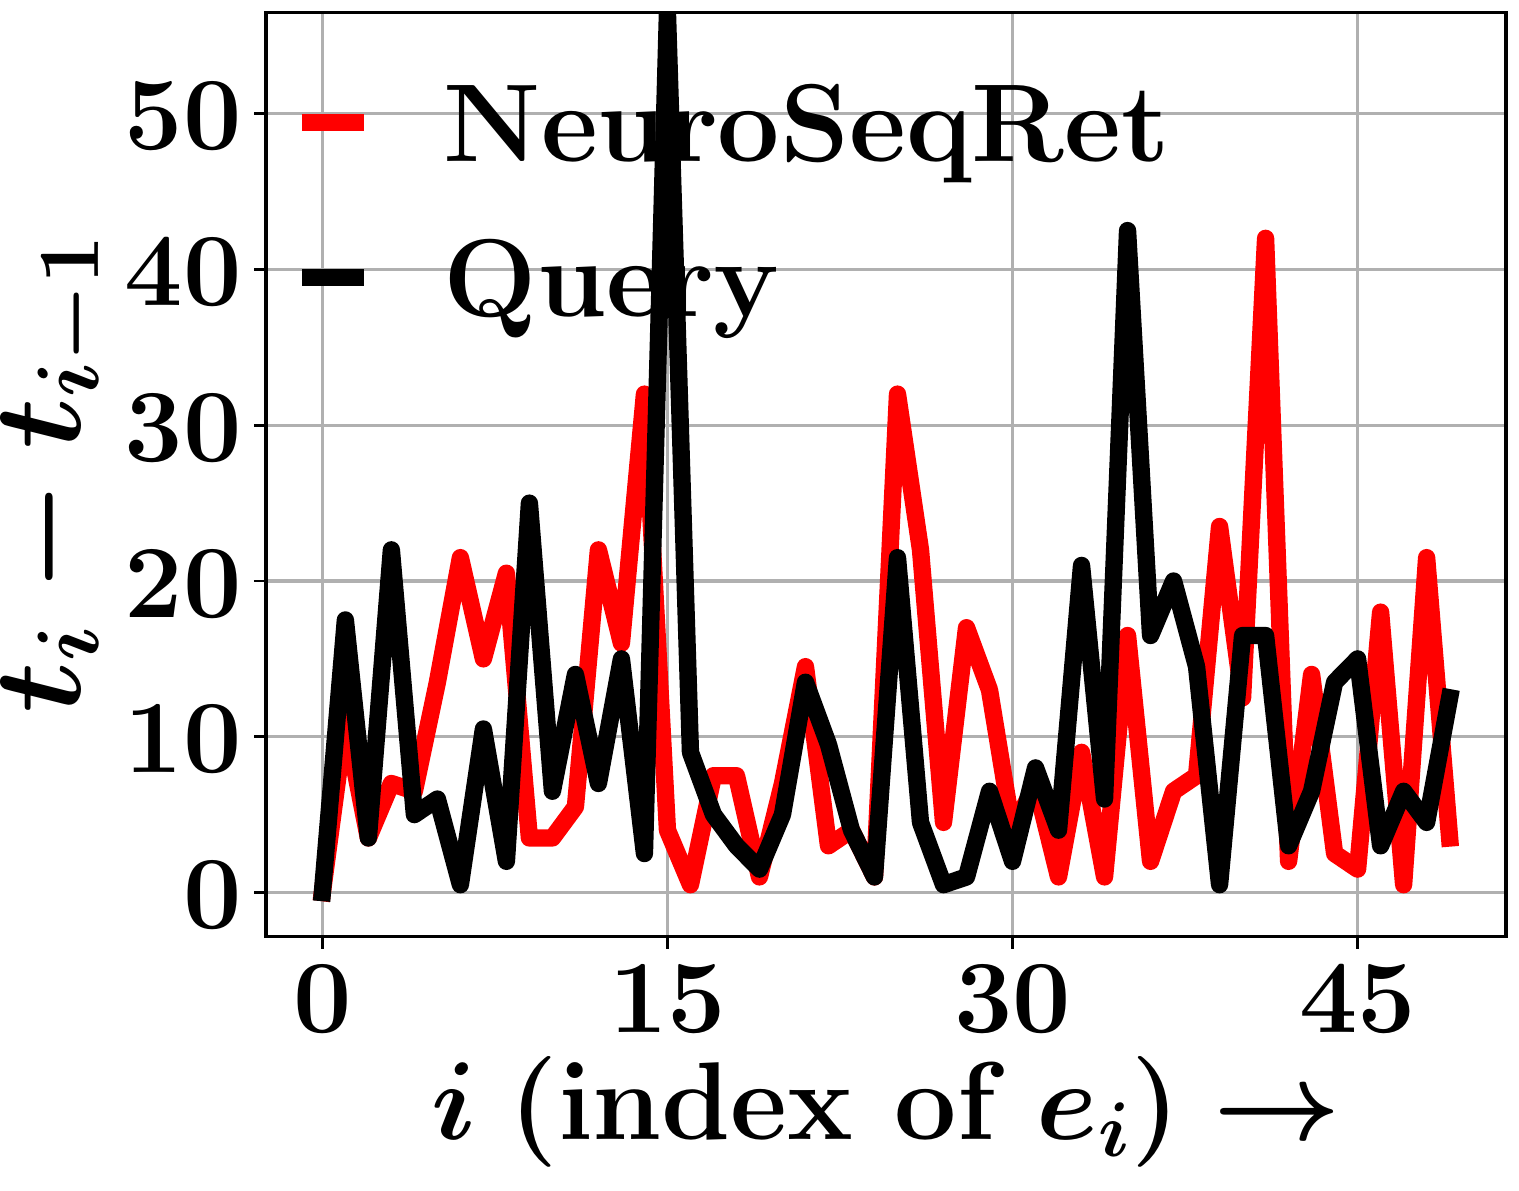}}
{\includegraphics[height=3cm]{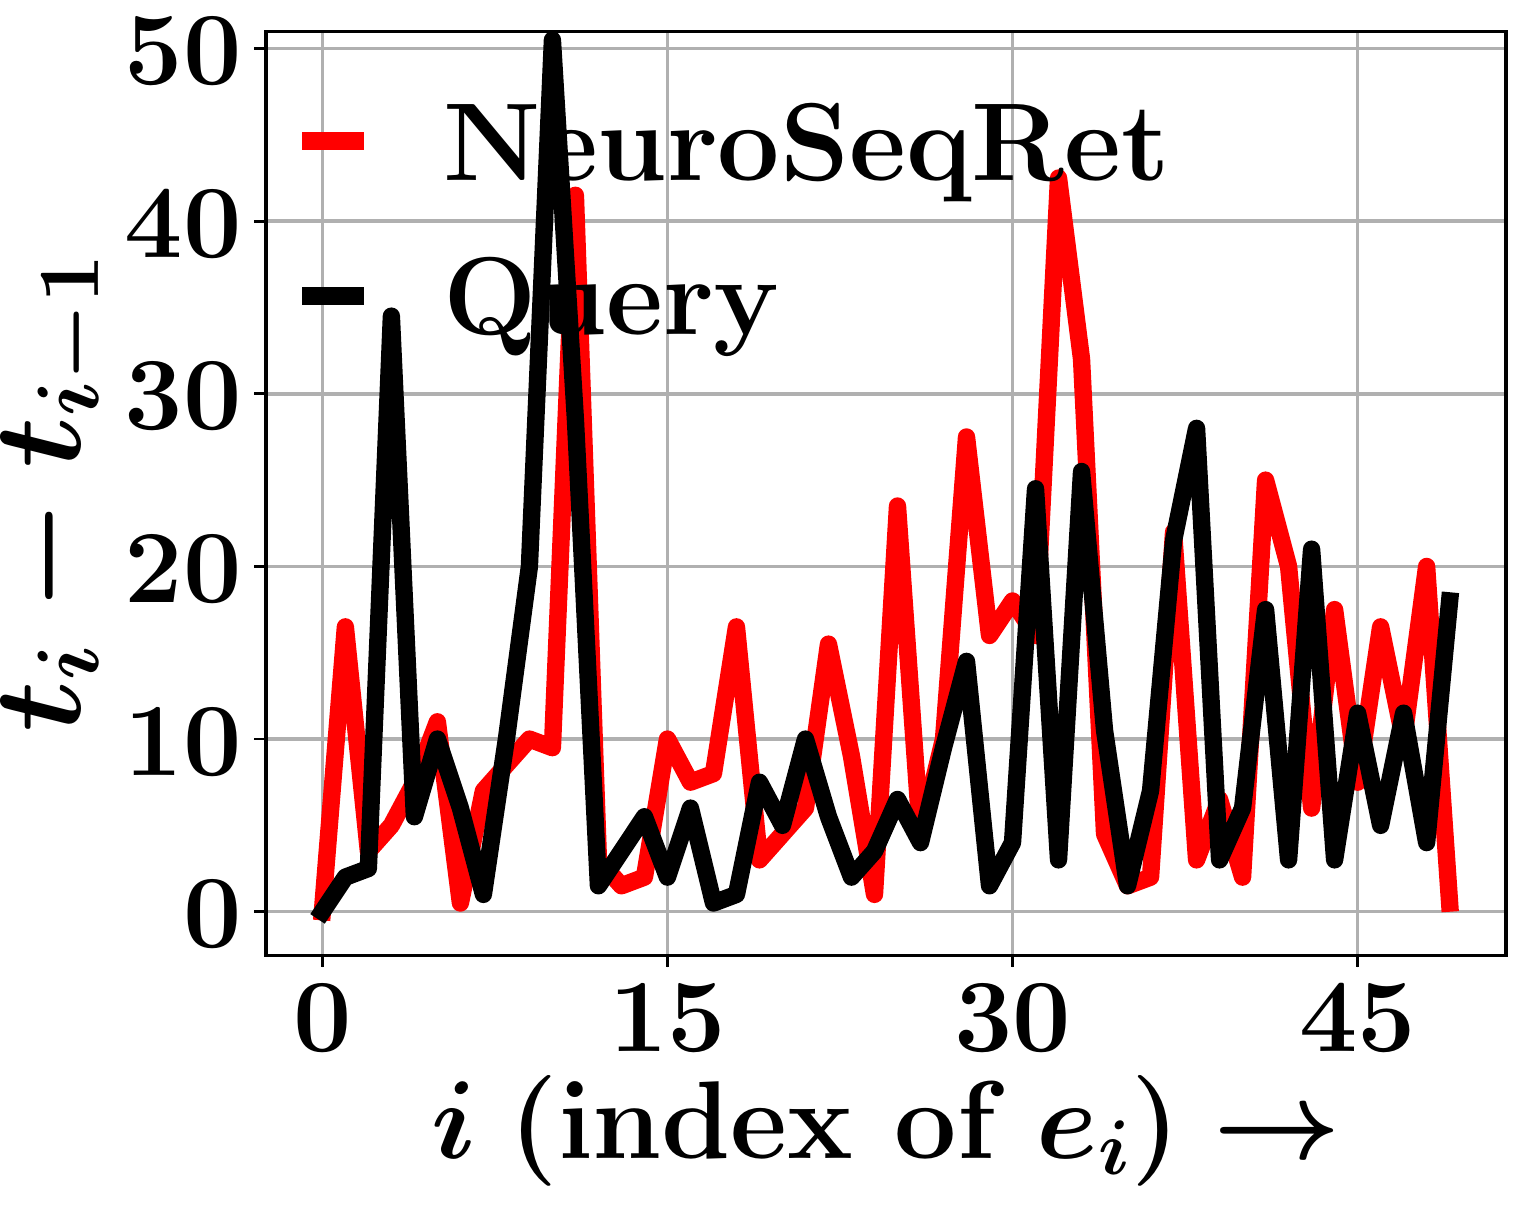}}
{\includegraphics[height=3cm]{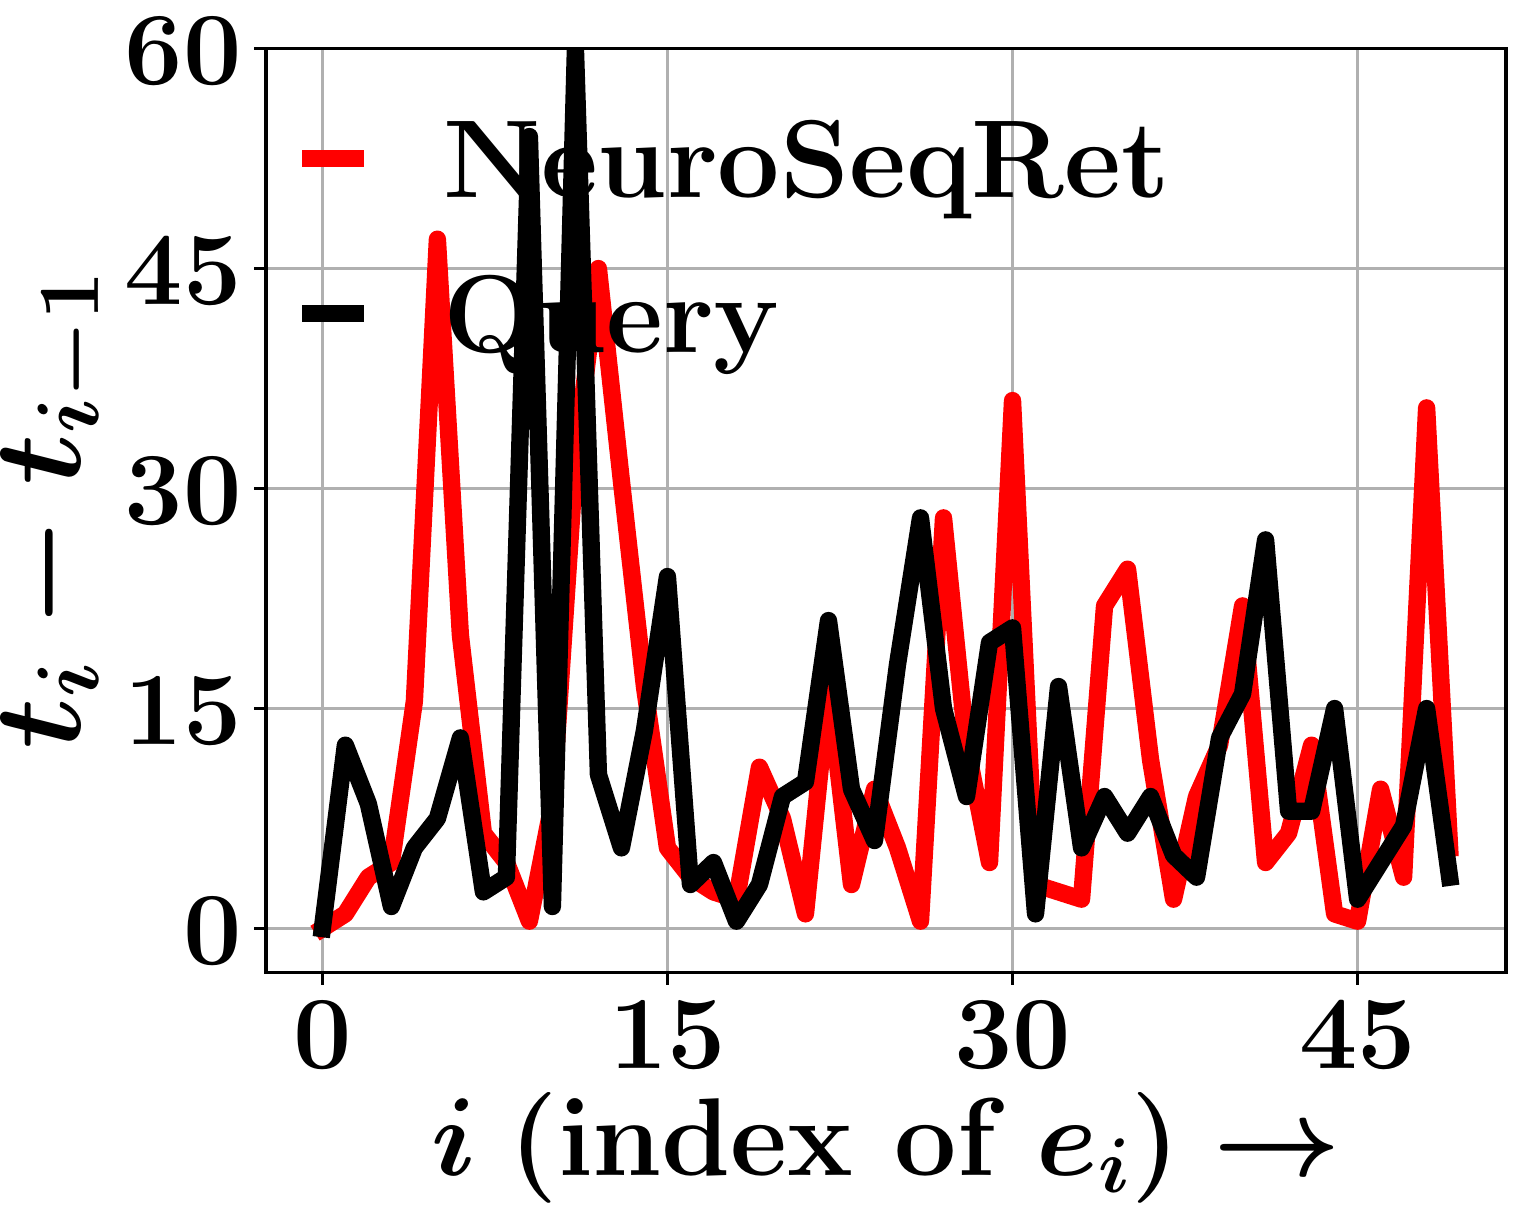}}
{\includegraphics[height=3cm]{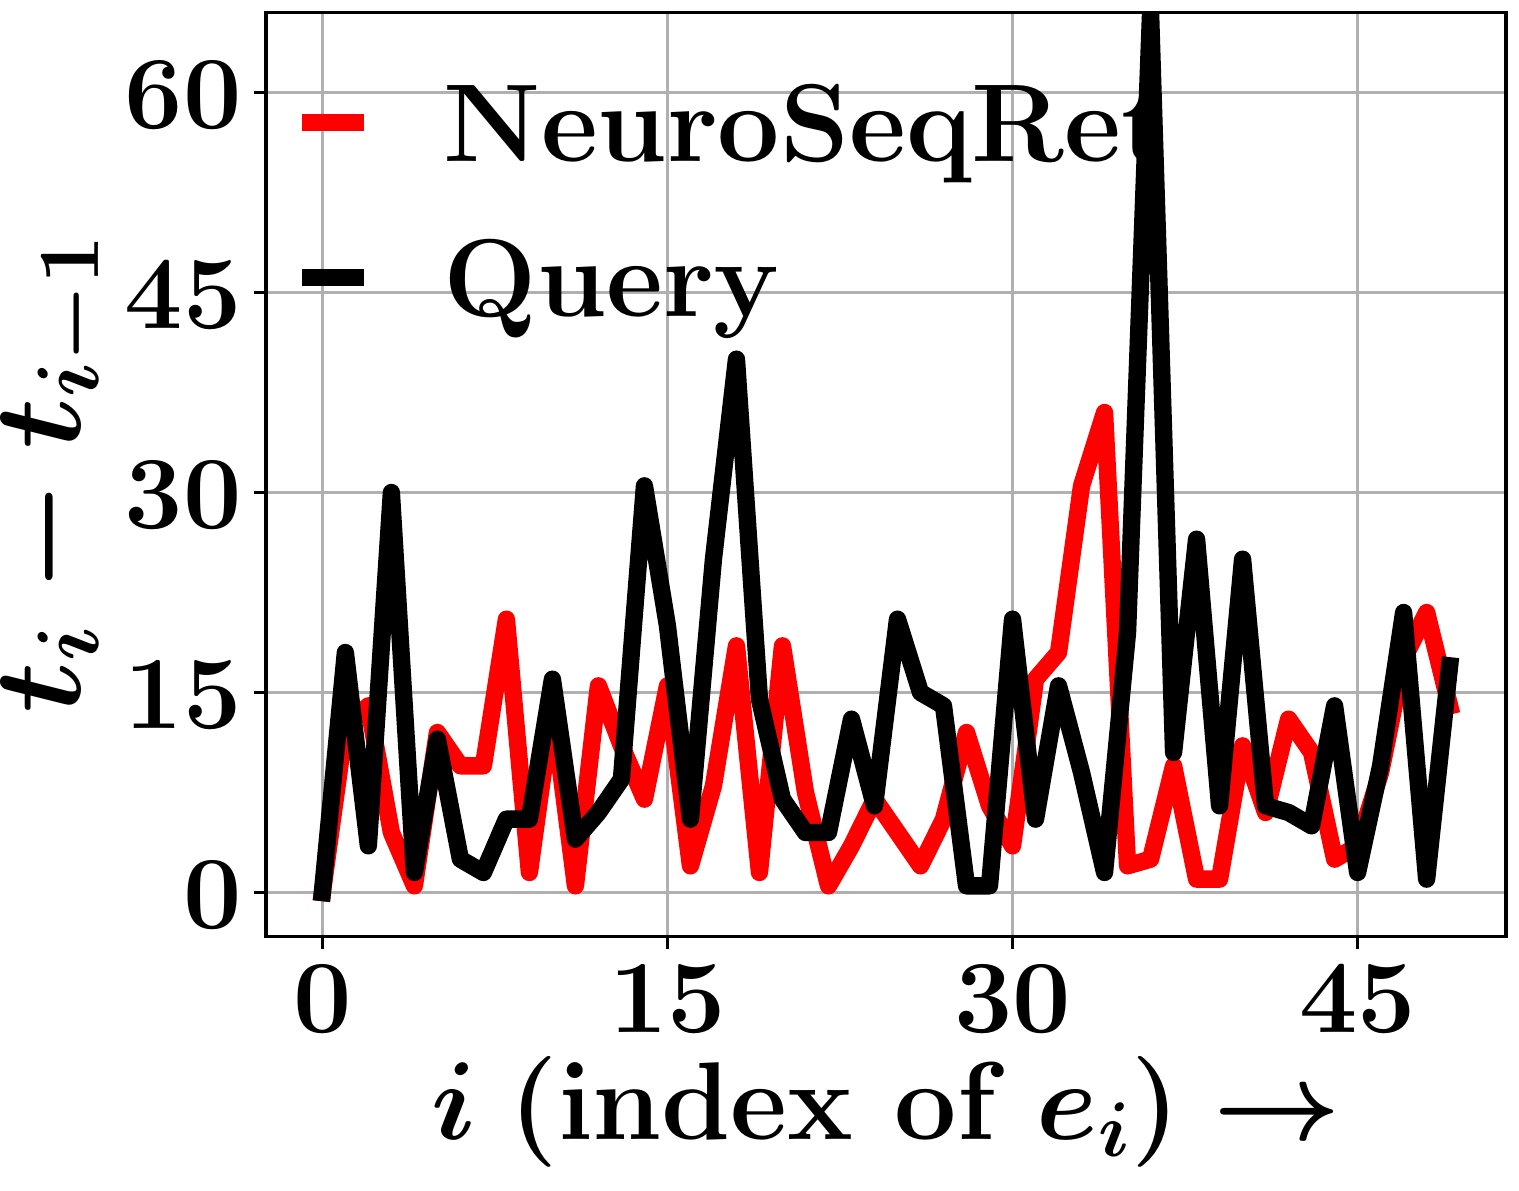}}

\subfloat[Sports dataset]
 {\includegraphics[height=3cm]{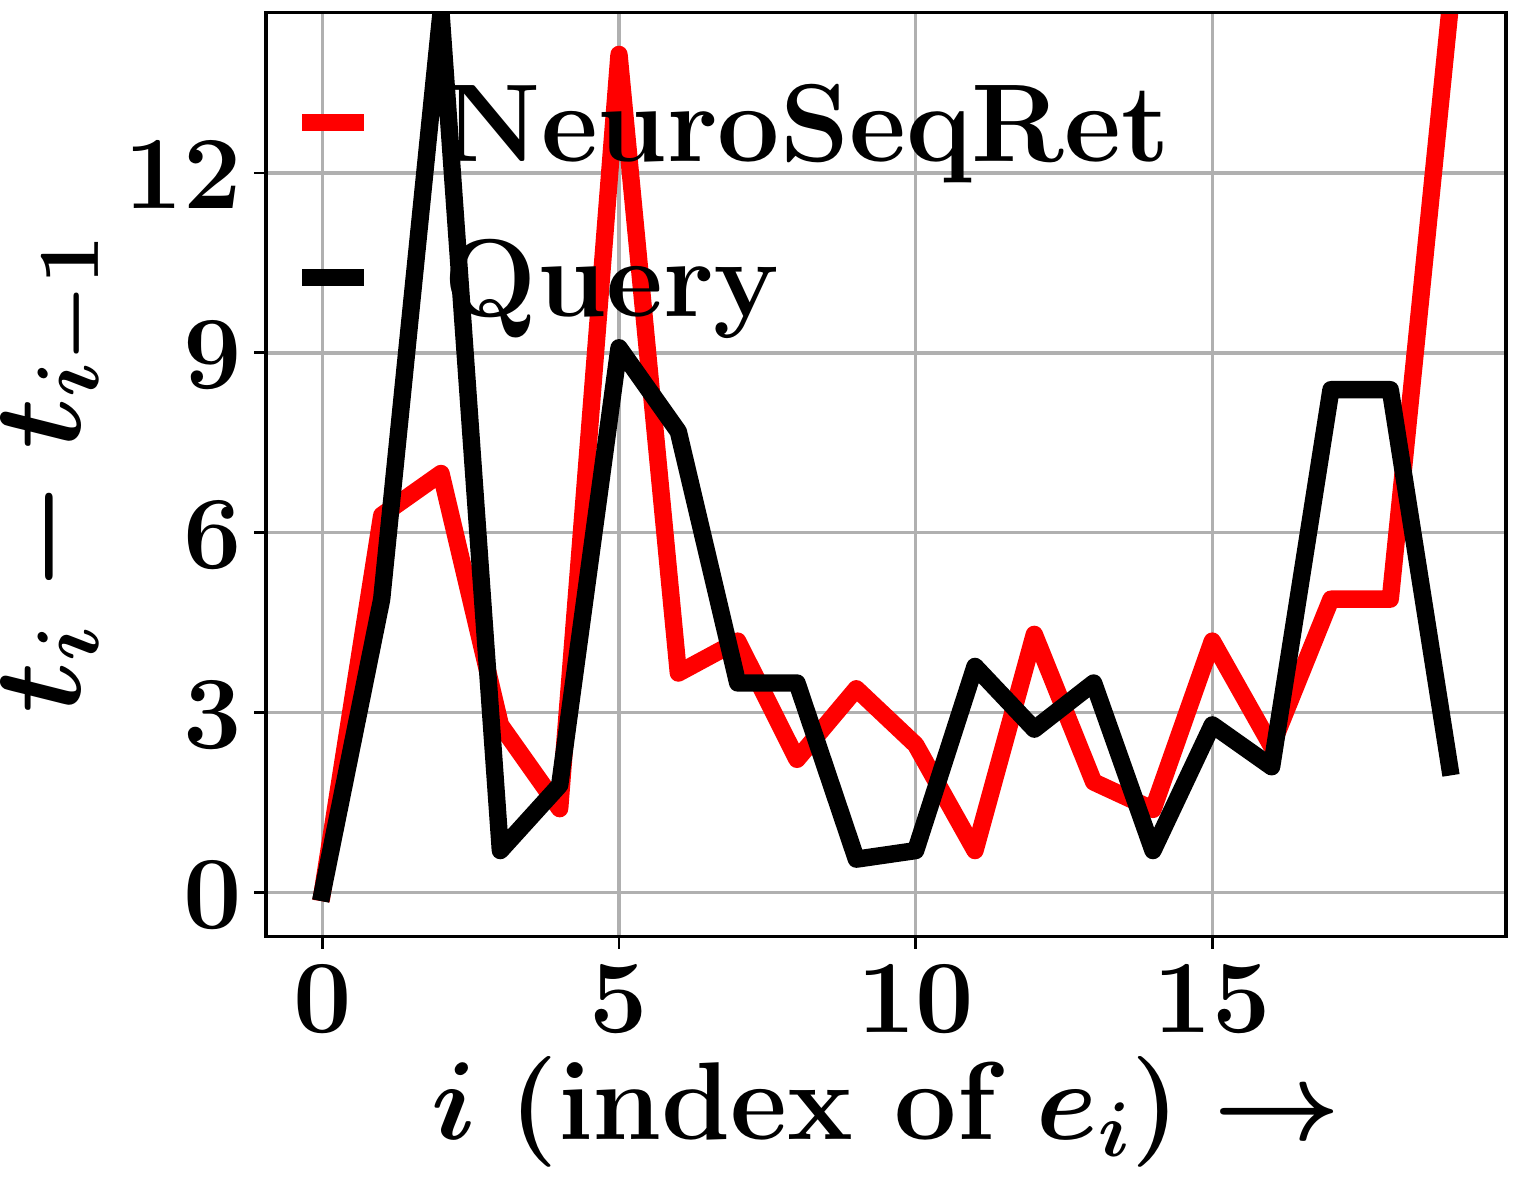}}
 {\includegraphics[height=3cm]{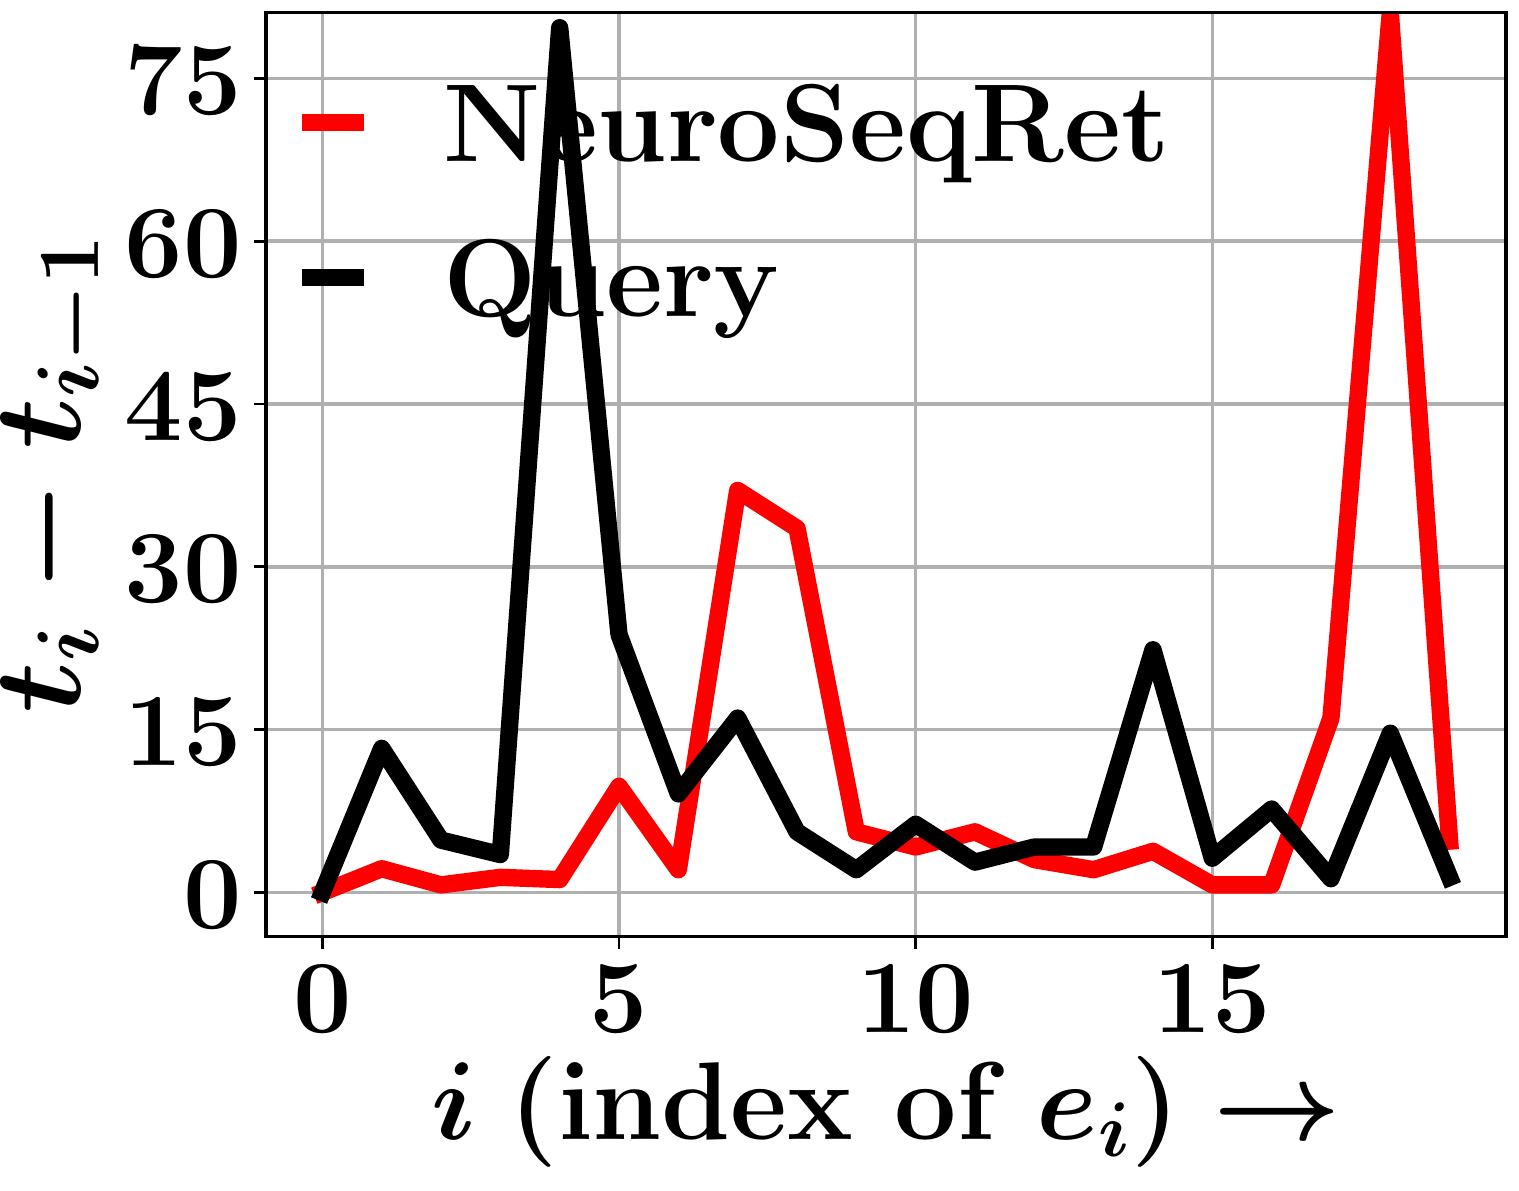}}
 {\includegraphics[height=3cm]{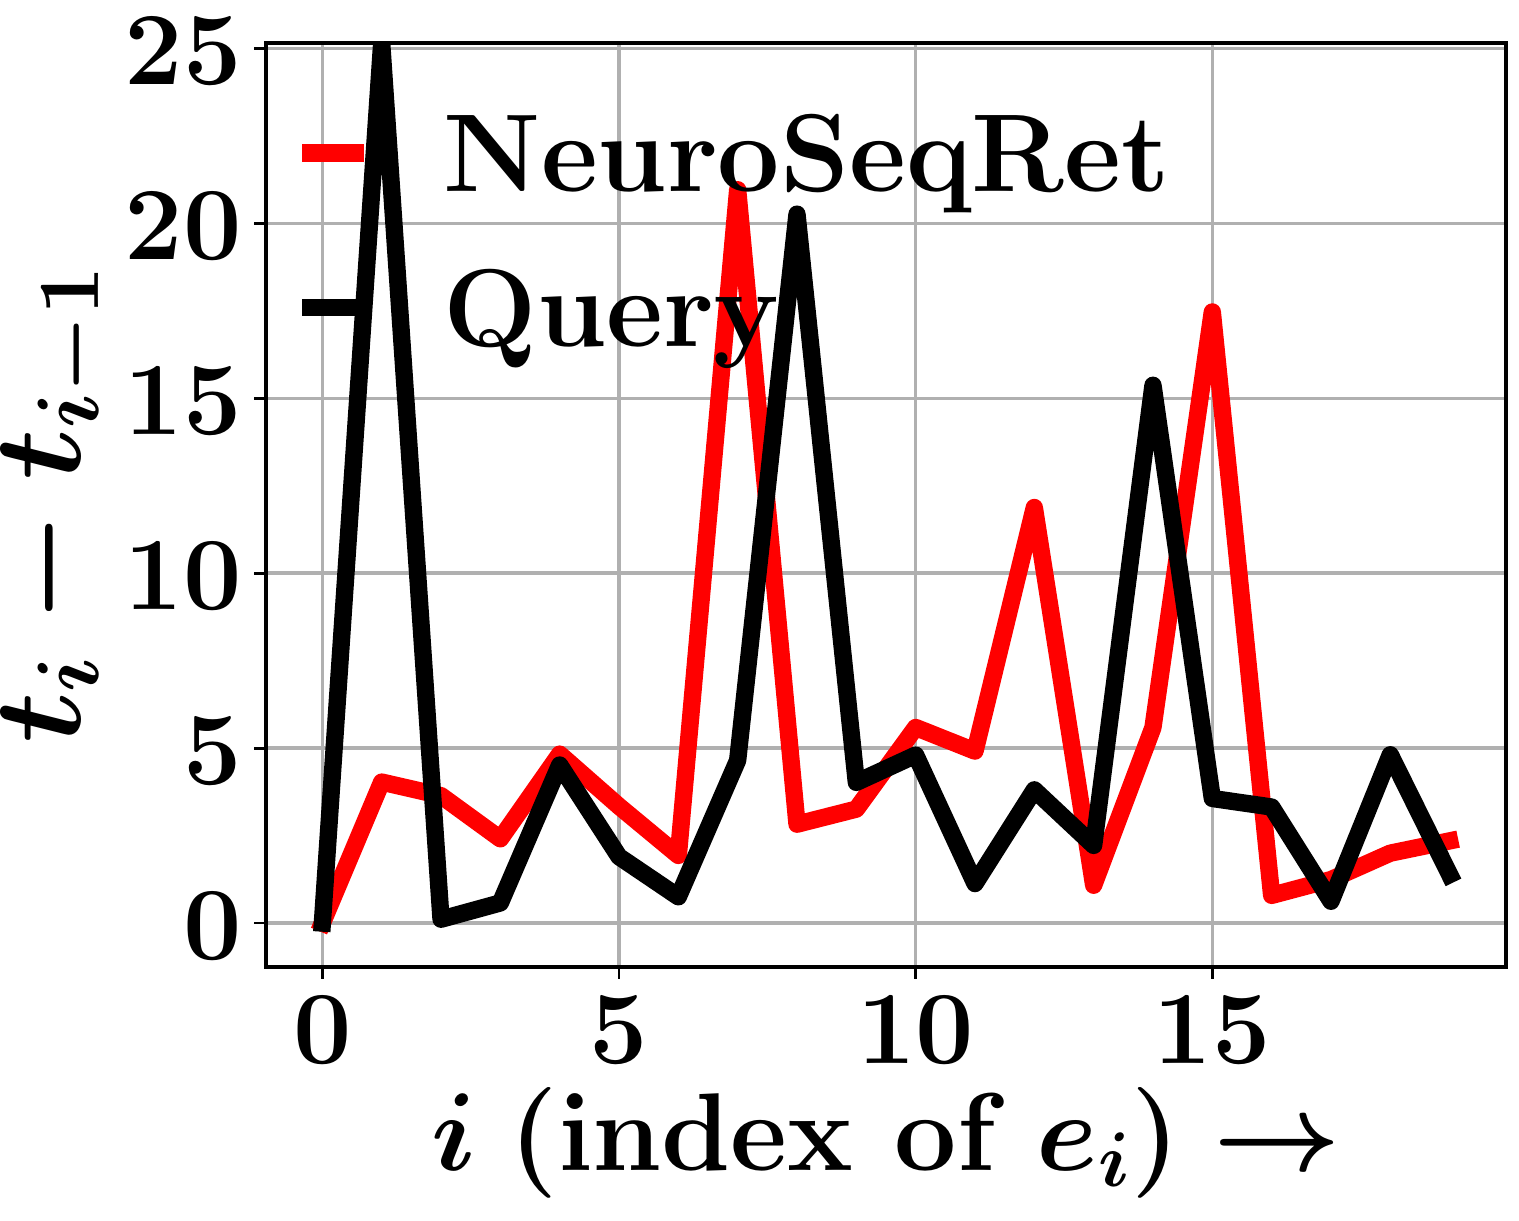}}
 {\includegraphics[height=3cm]{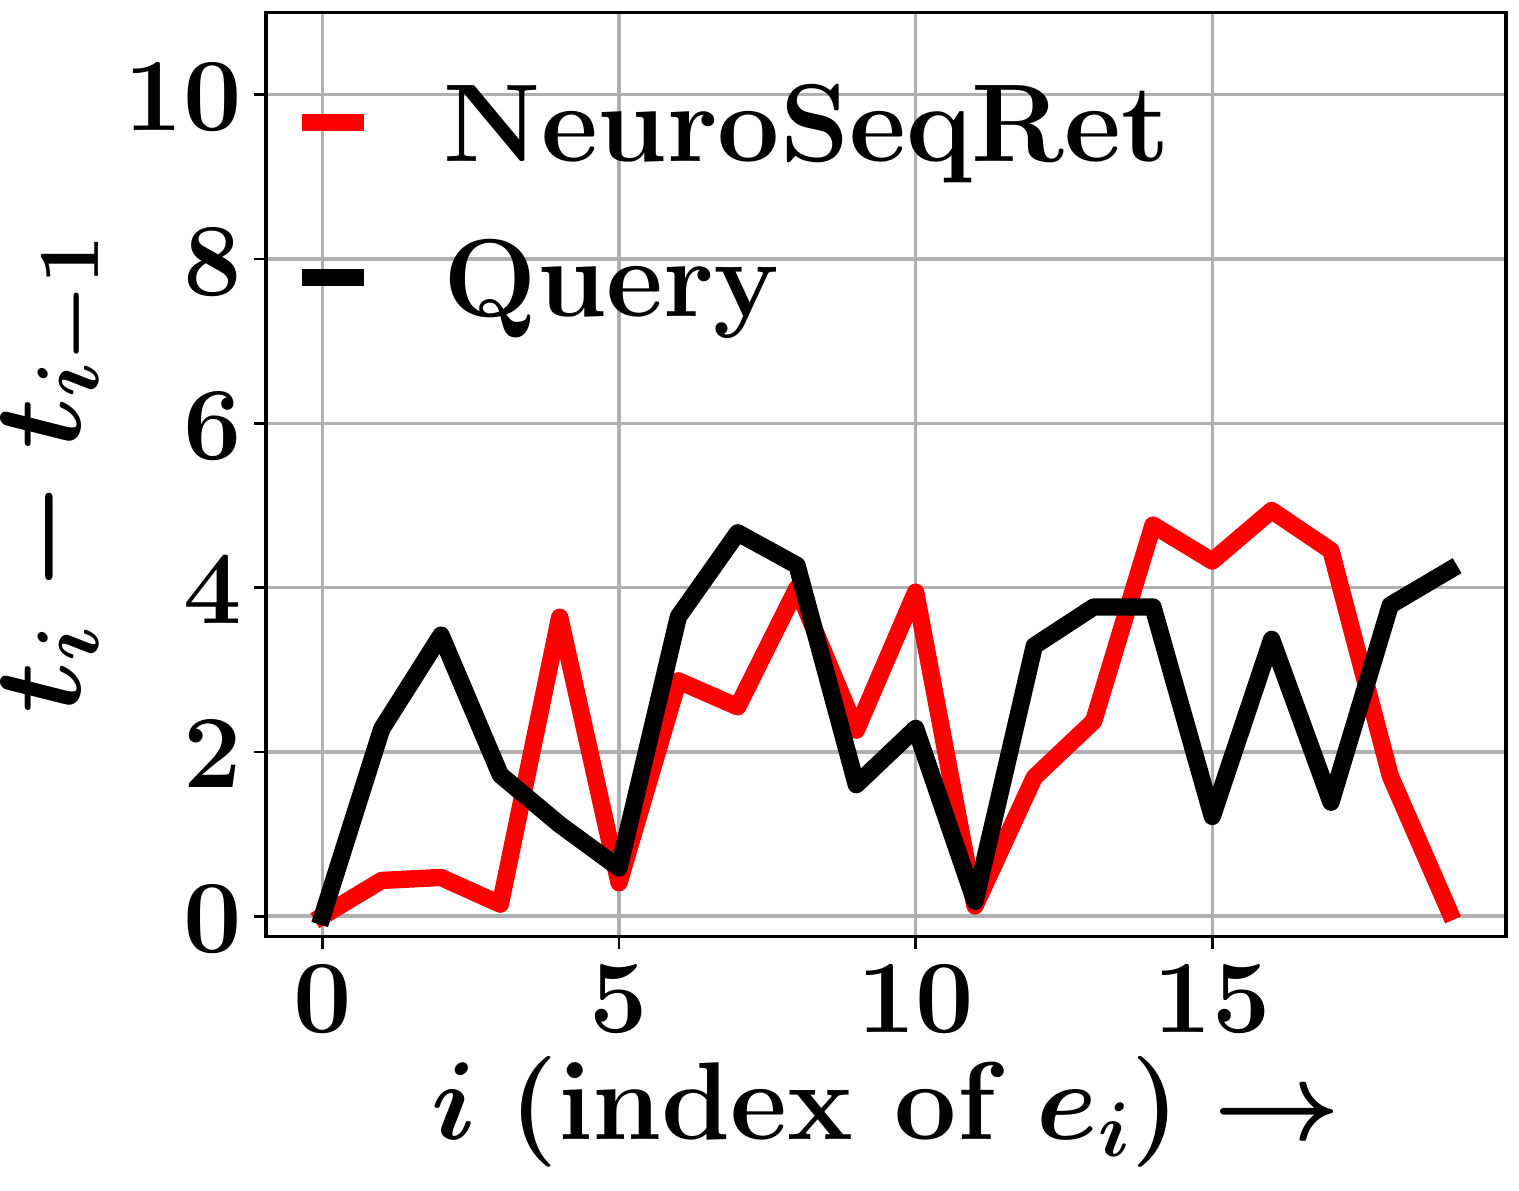}}
\caption{Qualitative examples of inter-event times of events in a query sequence and the top-search results by \our for all datasets.}
\label{fig:qualitative}
\end{figure}
%\section{Broader impact} \label{app:impact}
%Existing temporal point process models have shown great potential in modeling continuous-time event sequences across different domains -- from social networks to healthcare~\cite{Valera2014,rizoiu2017expecting,wang2017human}. Our proposed model is the first approach to introduce TPP models for retrieving sequences. We believe that our work will have a considerable impact on problems related to searching for trending topics, misinformation management in which, one may use our model to search relevance between diffusion processes of fake contents, stock market prediction in which, one may use our model to estimate the profit/loss based on the relevance between current market trends and the trends observed in the past. 
%
%However, as described before, our proposed model does not automatically preserve the privacy of a user.
%It would be interesting to devise a differentially private retrieval model as future work.
%As stated in Section~\ref{sec:conclusions}, in critical applications like healthcare, it would be important to use human interventions to mitigate risks that can have adverse impact~\cite{mozannar2020consistent}. 
%Finally, the proposed model also does not consider \textit{fairness} in ranking sequences, a crucial aspect of modern retrieval systems.
